# Supplementary material for: Bayesian multi-objective optimization for stochastic simulators: an extension of the Pareto Active Learning method
Source: arXiv:2207.03842 source file (2022-07-20)
Supplement: Supplementary file 1 [file barracosa-pals-suppmat.pdf]

Supplementary material for:

# “Bayesian multi-objective optimization for stochastic simulators: an extension of the Pareto Active Learning method”

Bruno Barracosa[a,b], Julien Bect[b], Héloïse Dutrieux Baraffe[a], Juliette Morin[a], Josselin Fournel[a], Emmanuel Vazquez[b,*]

[a] *EDF R&D, Power Systems and Energy Markets (SYSTEME), Palaiseau, France*
[b] *Université Paris-Saclay, CNRS, CentraleSupélec, Laboratoire des signaux et systèmes, 91190, Gif-sur-Yvette, France.*

**Abstract**

This document presents the numerical experiments described in the article “Bayesian multi-objective optimization for stochastic simulators: an extension of the Pareto Active Learning method”.

This document is organized as follows:

1. Influence of the parameter $\beta$ of PALS.
2. Influence of the parameter $\varepsilon$ of PALS.
3. Using intersections in PALS.
4. Influence of the batch size.
5. Comparison of two random-based proposed alternatives.
6. Comparison with other approaches.

## 1. Influence of the parameter $\beta$ of PALS

The average volume of the symmetric difference for problems $g_1$ to $g_9$ is illustrated in figures 1 to 18 for the three different noise levels considered.

While figures 19 to 36 illustrate the classification error metric, for the same problems $g_1$ to $g_9$ for the three different noise levels considered.

*Corresponding author
*Email address:* emmanuel.vazquez@centralesupelec.fr (Emmanuel Vazquez)

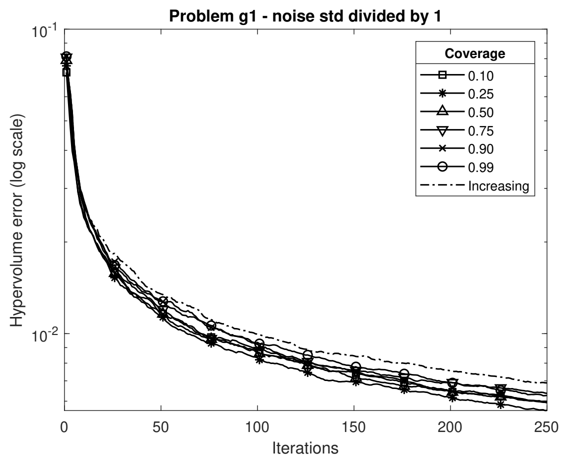


Figure 1: Average volume of the symmetric difference for problem $g_1$ for different $\beta$ values

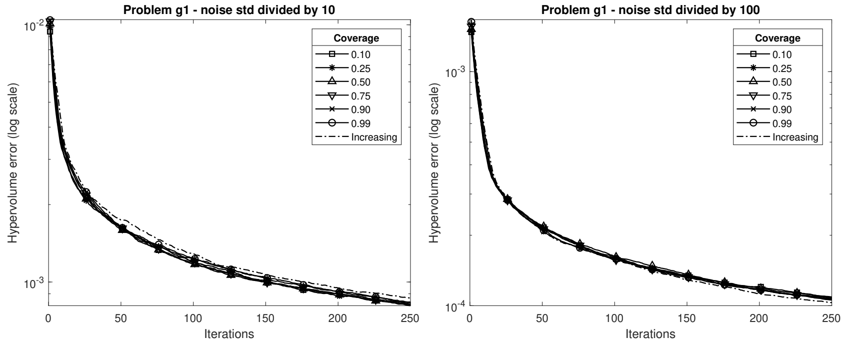


Figure 2: Average volume of the symmetric difference for problem $g_1$ for different $\beta$ values, with the problem noise standard deviation divided by 10 (left) and by 100 (right)

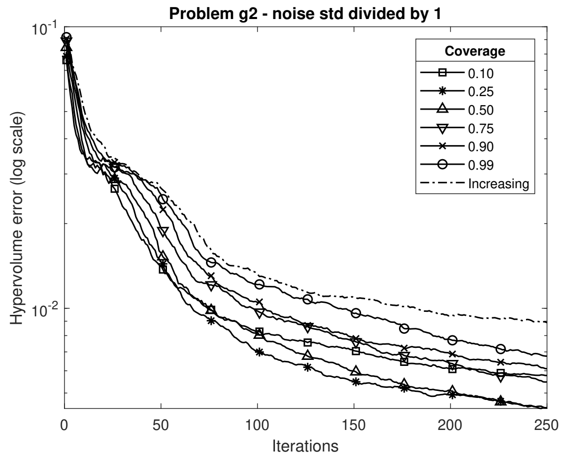


Figure 3: Average volume of the symmetric difference for problem $g_2$ for different $\beta$ values

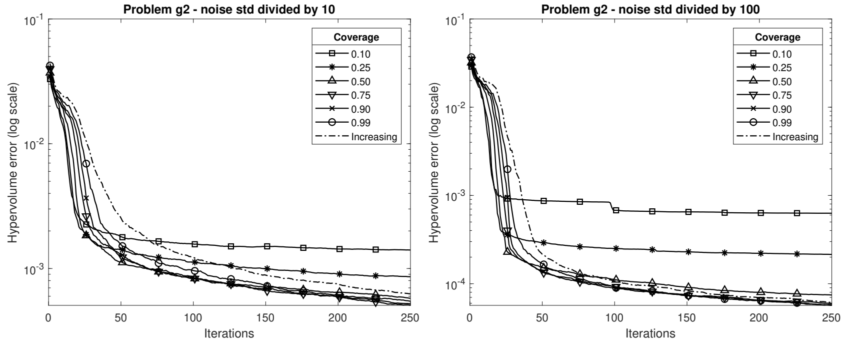


Figure 4: Average volume of the symmetric difference for problem $g_2$ for different $\beta$ values, with the problem noise standard deviation divided by 10 (left) and by 100 (right)

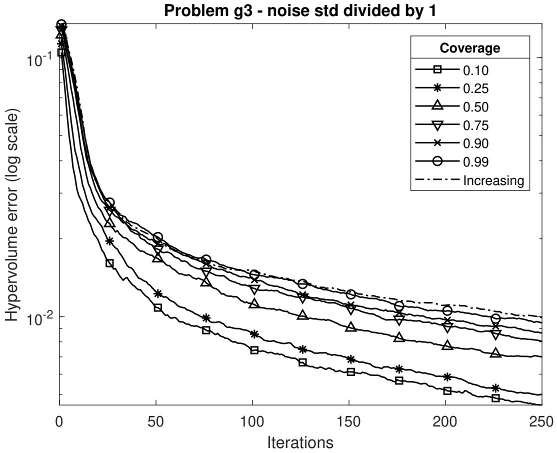


Figure 5: Average volume of the symmetric difference for problem $g_3$ for different $\beta$ values

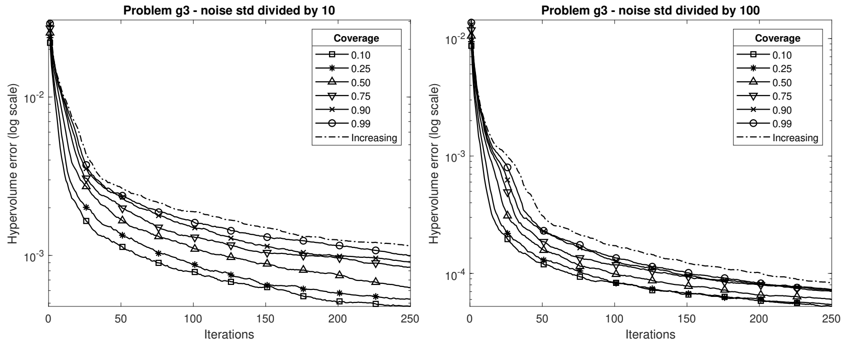


Figure 6: Average volume of the symmetric difference for problem $g_3$ for different $\beta$ values, with the problem noise standard deviation divided by 10 (left) and by 100 (right)

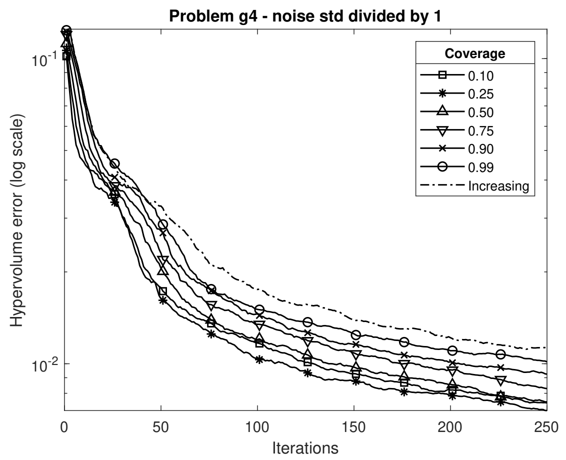


Figure 7: Average volume of the symmetric difference for problem $g_4$ for different $\beta$ values

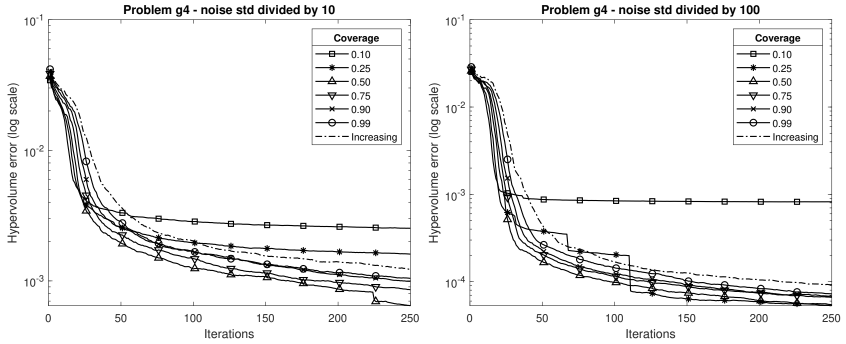


Figure 8: Average volume of the symmetric difference for problem $g_4$ for different $\beta$ values, with the problem noise standard deviation divided by 10 (left) and by 100 (right)

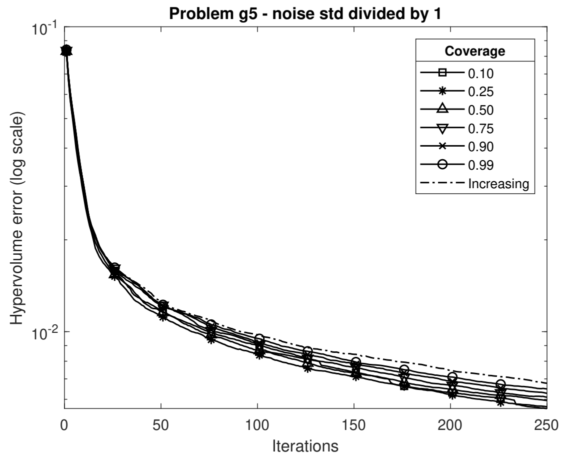


Figure 9: Average volume of the symmetric difference for problem $g_5$ for different $\beta$ values

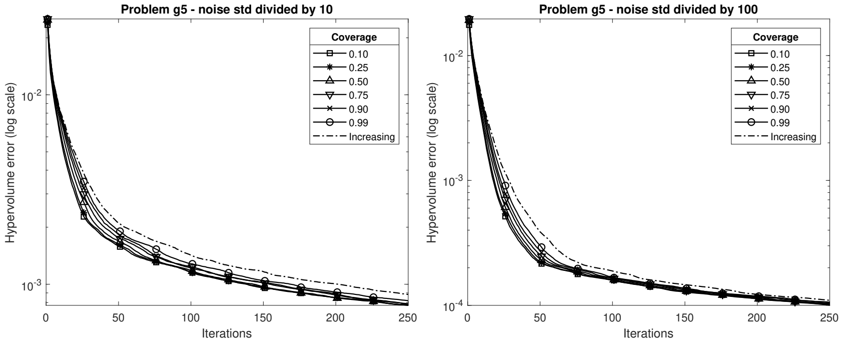


Figure 10: Average volume of the symmetric difference for problem $g_5$ for different $\beta$ values, with the problem noise standard deviation divided by 10 (left) and by 100 (right)

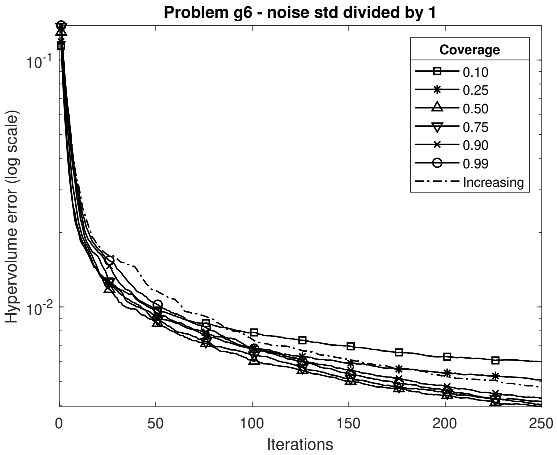


Figure 11: Average volume of the symmetric difference for problem $g_6$ for different $\beta$ values

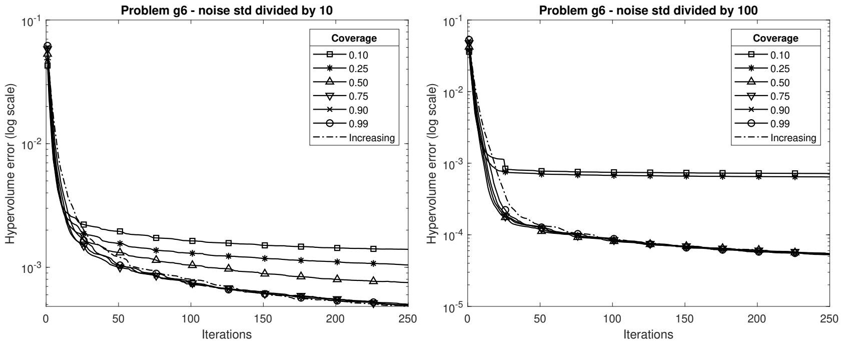


Figure 12: Average volume of the symmetric difference for problem $g_6$ for different $\beta$ values, with the problem noise standard deviation divided by 10 (left) and by 100 (right)

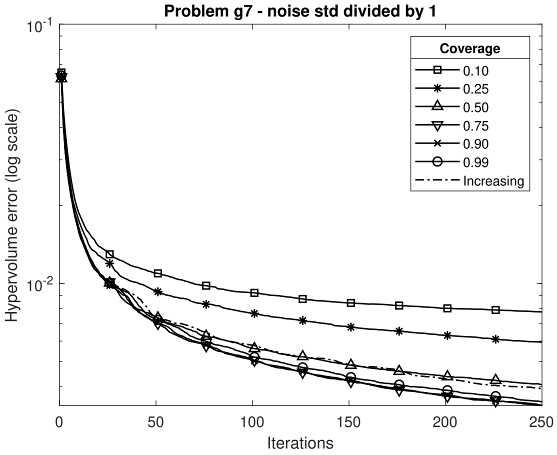


Figure 13: Average volume of the symmetric difference for problem $g_7$ for different $\beta$ values

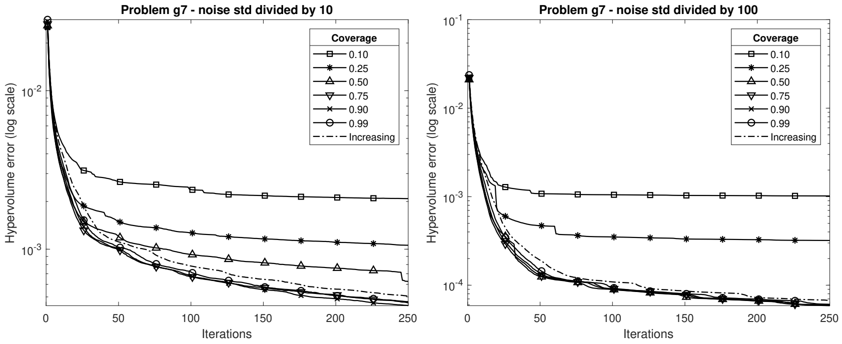


Figure 14: Average volume of the symmetric difference for problem $g_7$ for different $\beta$ values, with the problem noise standard deviation divided by 10 (left) and by 100 (right)

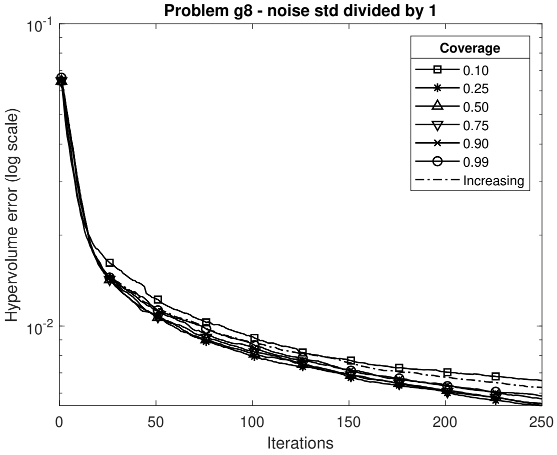


Figure 15: Average volume of the symmetric difference for problem $g_8$ for different $\beta$ values

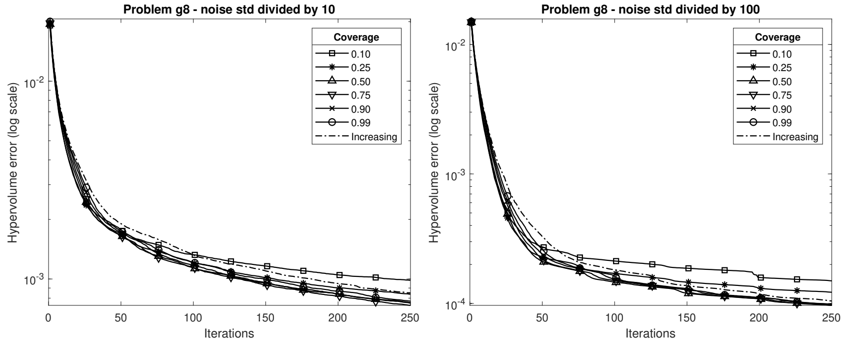


Figure 16: Average volume of the symmetric difference for problem $g_8$ for different $\beta$ values, with the problem noise standard deviation divided by 10 (left) and by 100 (right)

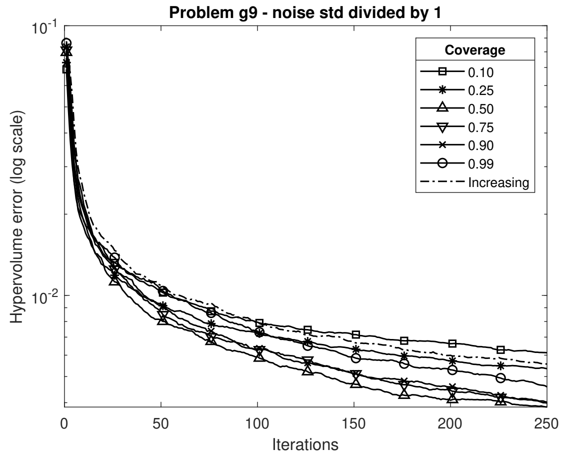


Figure 17: Average volume of the symmetric difference for problem $g_9$ for different $\beta$ values

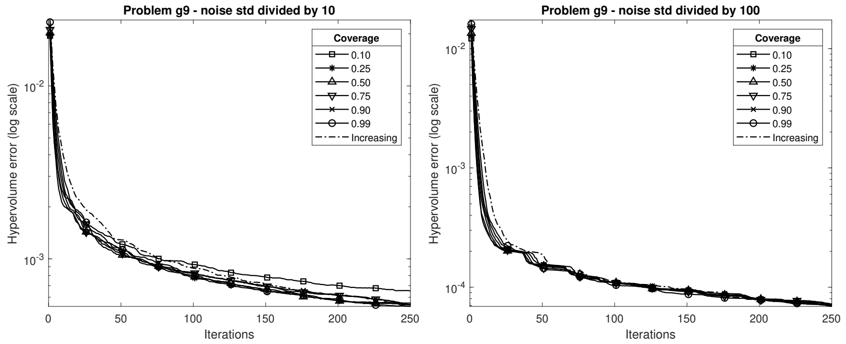


Figure 18: Average volume of the symmetric difference for problem $g_9$ for different $\beta$ values, with the problem noise standard deviation divided by 10 (left) and by 100 (right)

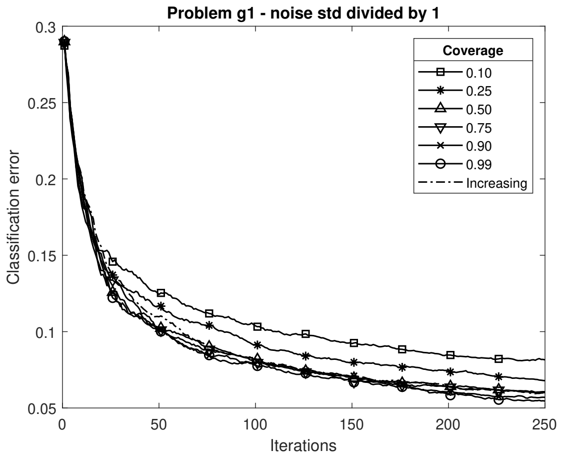


Figure 19: Classification error for problem $g_1$ for different $\beta$ values

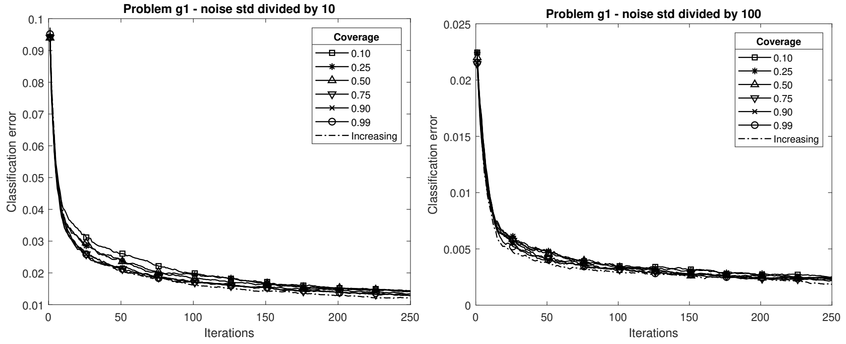


Figure 20: Classification error for problem $g_1$ for different $\beta$ values, with the problem noise standard deviation divided by 10 (left) and by 100 (right)

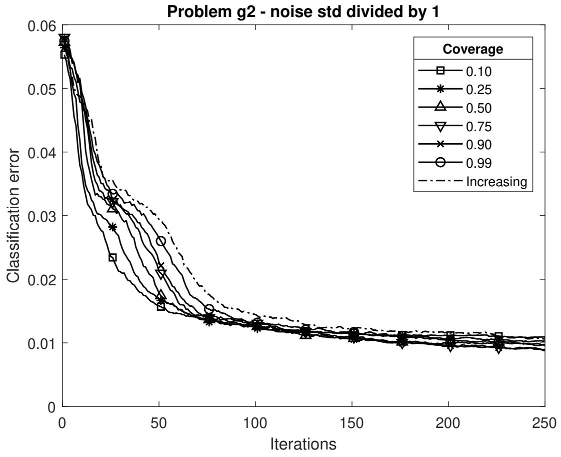


Figure 21: Classification error for problem $g_2$ for different $\beta$ values

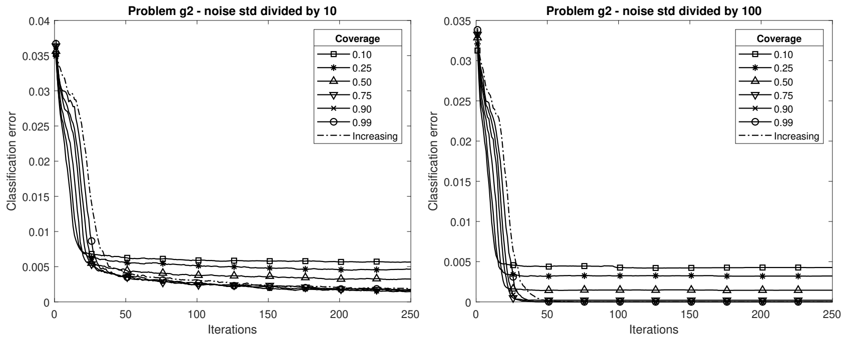


Figure 22: Classification error for problem $g_2$ for different $\beta$ values, with the problem noise standard deviation divided by 10 (left) and by 100 (right)

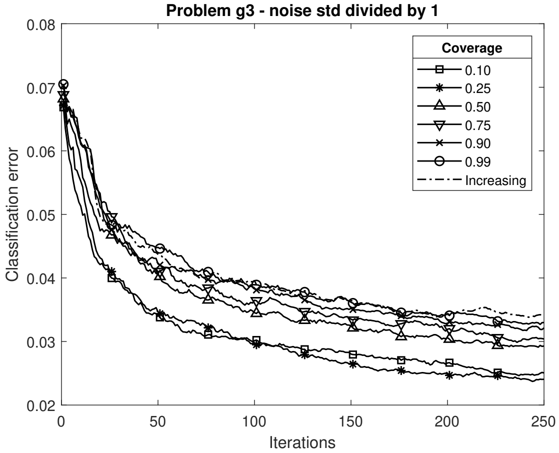


Figure 23: Classification error for problem $g_3$ for different $\beta$ values

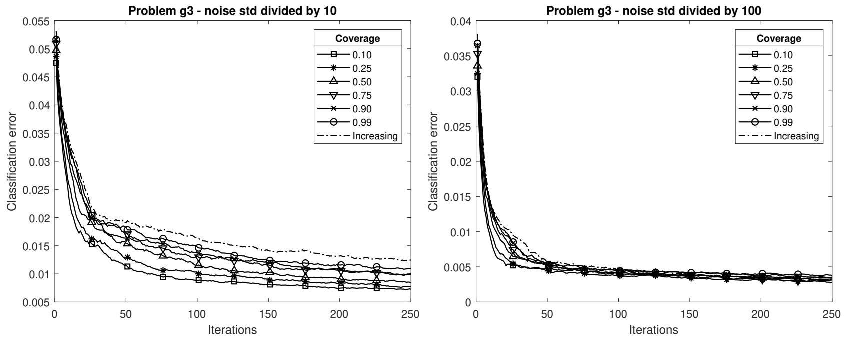


Figure 24: Classification error for problem $g_3$ for different $\beta$ values, with the problem noise standard deviation divided by 10 (left) and by 100 (right)

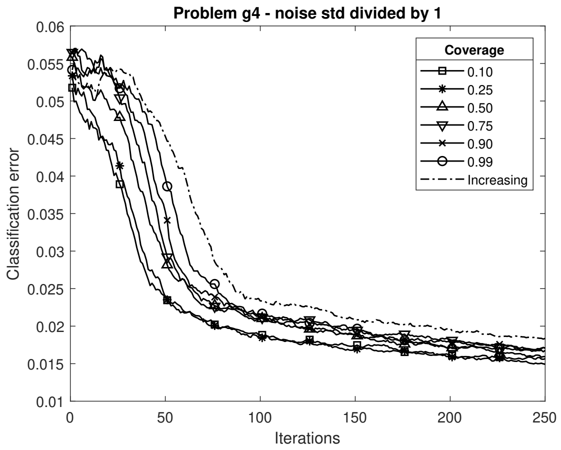


Figure 25: Classification error for problem $g_4$ for different $\beta$ values

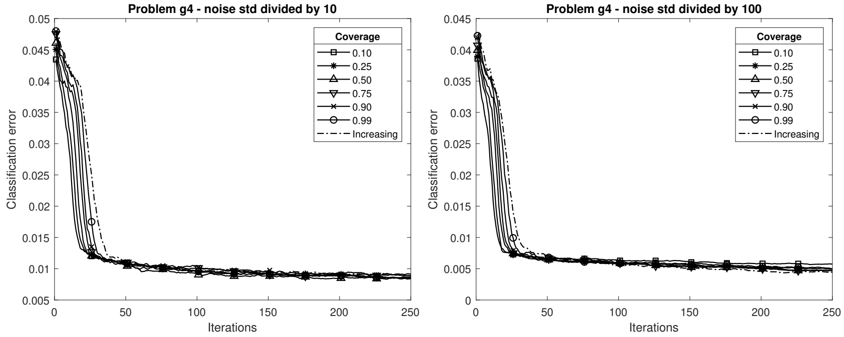


Figure 26: Classification error for problem $g_4$ for different $\beta$ values, with the problem noise standard deviation divided by 10 (left) and by 100 (right)

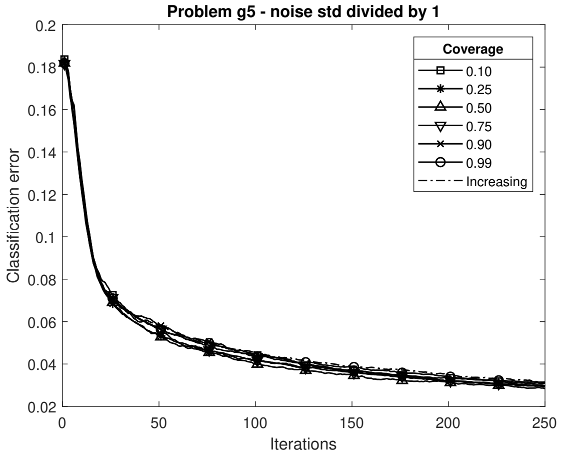


Figure 27: Classification error for problem $g_5$ for different $\beta$ values

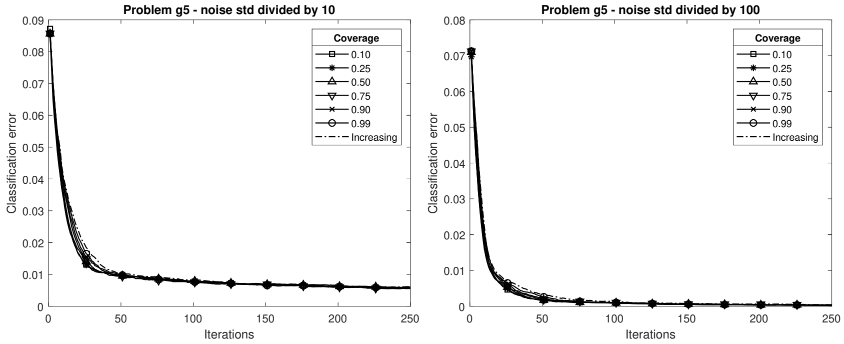


Figure 28: Classification error for problem $g_5$ for different $\beta$ values, with the problem noise standard deviation divided by 10 (left) and by 100 (right)

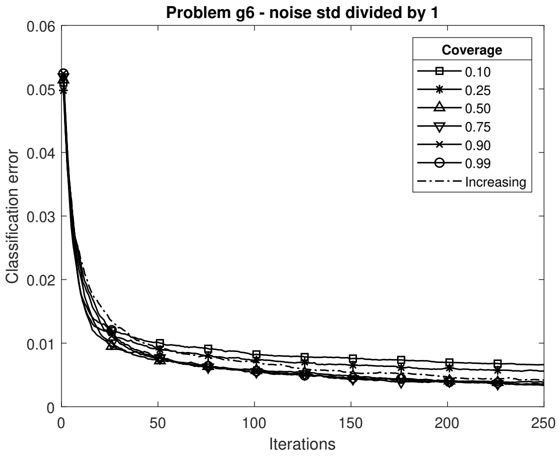


Figure 29: Classification error for problem $g_6$ for different $\beta$ values

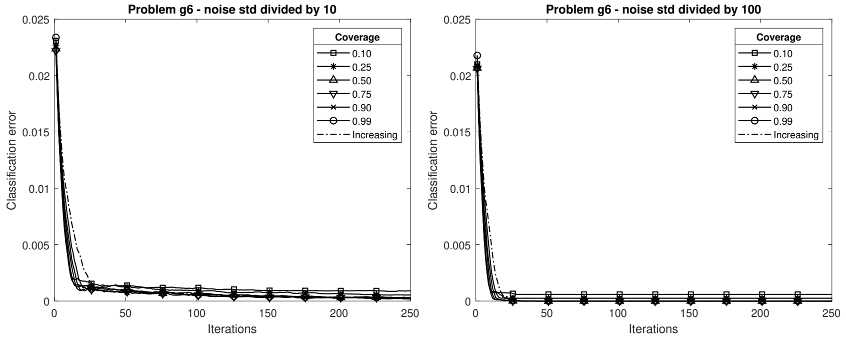


Figure 30: Classification error for problem $g_6$ for different $\beta$ values, with the problem noise standard deviation divided by 10 (left) and by 100 (right)

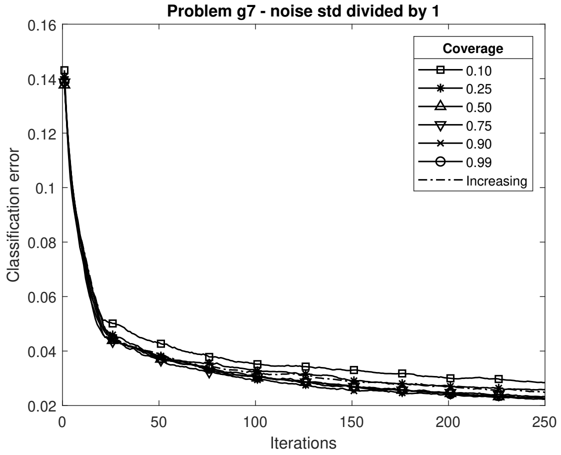


Figure 31: Classification error for problem $g_7$ for different $\beta$ values

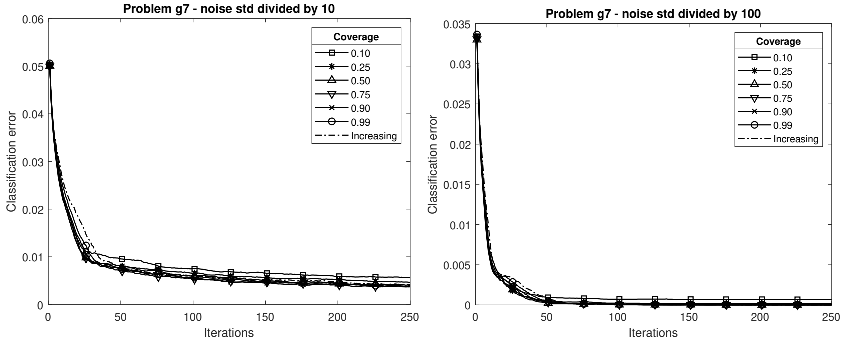


Figure 32: Classification error for problem $g_7$ for different $\beta$ values, with the problem noise standard deviation divided by 10 (left) and by 100 (right)

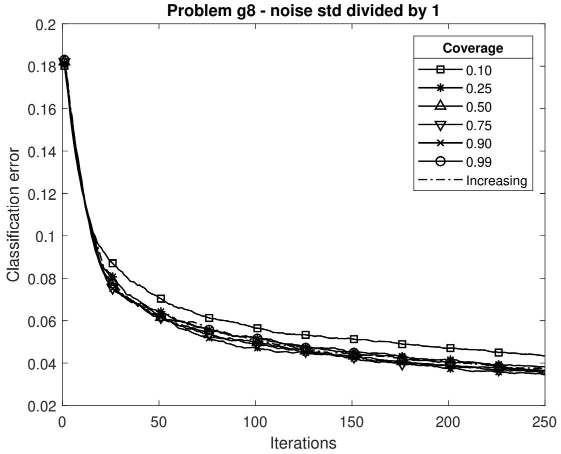


Figure 33: Classification error for problem $g_8$ for different $\beta$ values

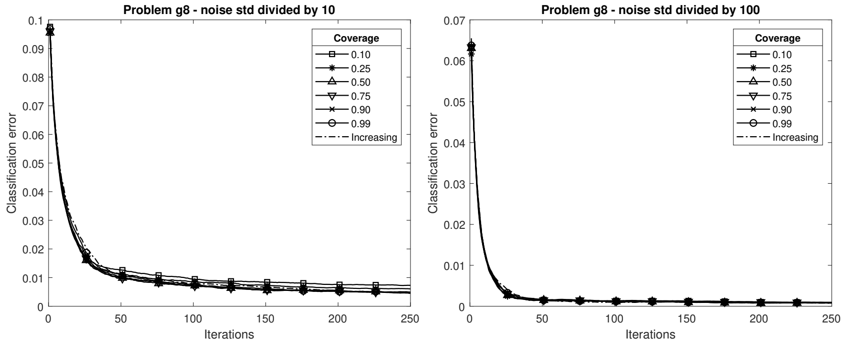


Figure 34: Classification error for problem $g_8$ for different $\beta$ values, with the problem noise standard deviation divided by 10 (left) and by 100 (right)

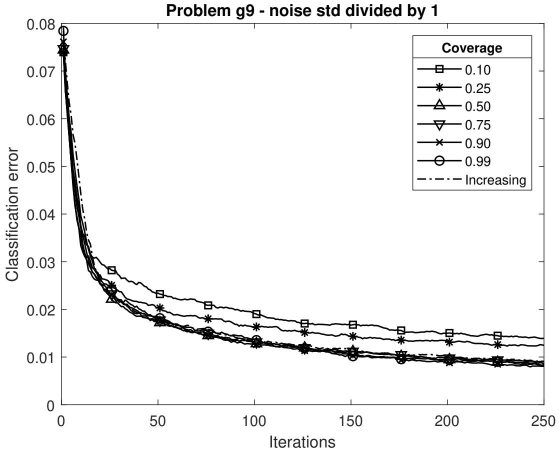


Figure 35: Classification error for problem $g_9$ for different $\beta$ values

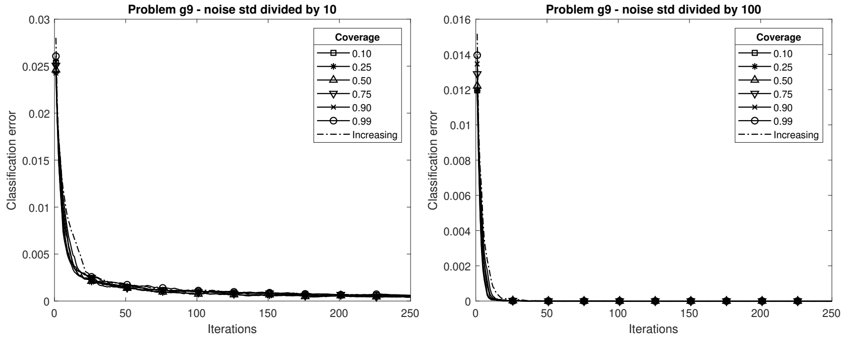


Figure 36: Classification error for problem $g_9$ for different $\beta$ values, with the problem noise standard deviation divided by 10 (left) and by 100 (right)

## 2. Influence of the parameter $\varepsilon$ of PALS

When considering the impact of $\varepsilon$ on the metric value, at final iteration, the result for the average volume of the symmetric difference is presented in Figure 37, while the average classification error in figure 38.

The average metrics evolution, for problems $g_1$ to $g_9$, for the different $\varepsilon$ values is presented in Figures 39 to 47 for the average volume of the symmetric difference metric, in Figures 48 to 56 for the average classification error metric, in Figures 57 to 65 for the average Hausdorff distance of the Pareto front prediction, and in Figures 66 to 74 for the average Hausdorff distance of the Pareto set prediction.

The use of $\varepsilon$ allows establishing a trade-off between accurate prediction and classification speed. To illustrate classification speed, Figures 75 to 83 present the evolution of the average cardinality of the unclassified set for each problem, for different values of $\varepsilon$.

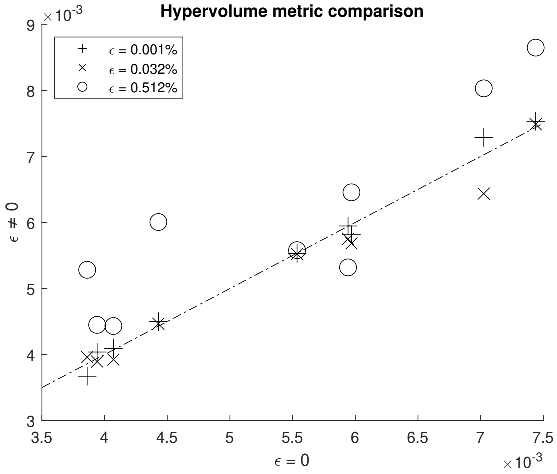


Figure 37: Average volume of the symmetric difference at final iteration for all the problems, for different $\varepsilon$ choices when compared to $\varepsilon = 0$.

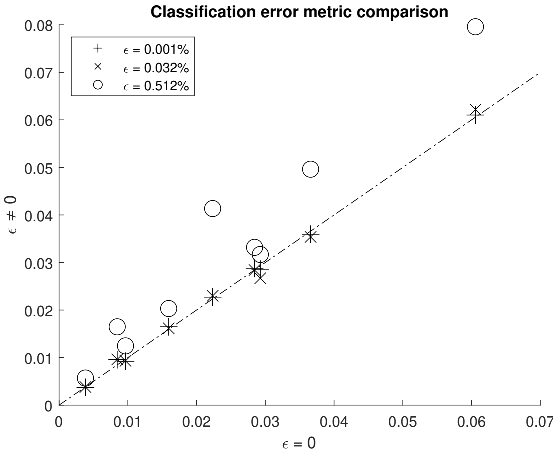


Figure 38: Average classification error at final iteration for all the problems, for different $\varepsilon$ choices when compared to $\varepsilon = 0$.

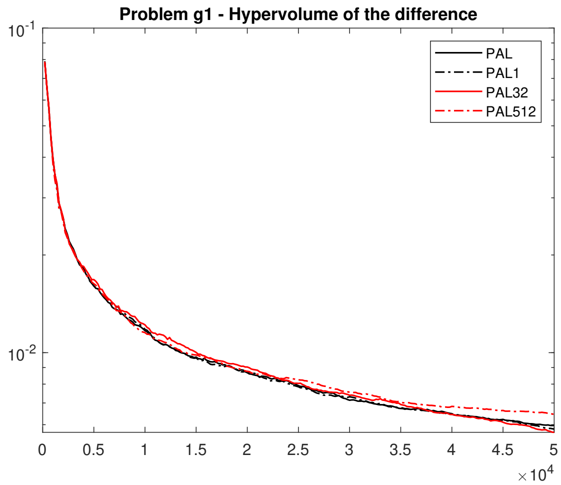


Figure 39: Average volume of the symmetric difference metric for problem $g_1$ for different $\varepsilon$ values.

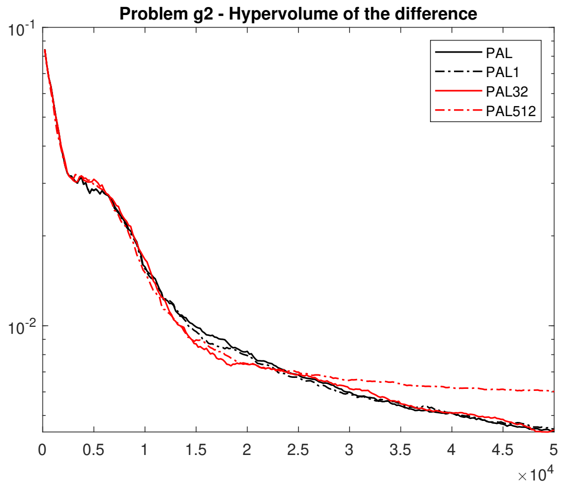


Figure 40: Average volume of the symmetric difference metric for problem $g_2$ for different $\varepsilon$ values.

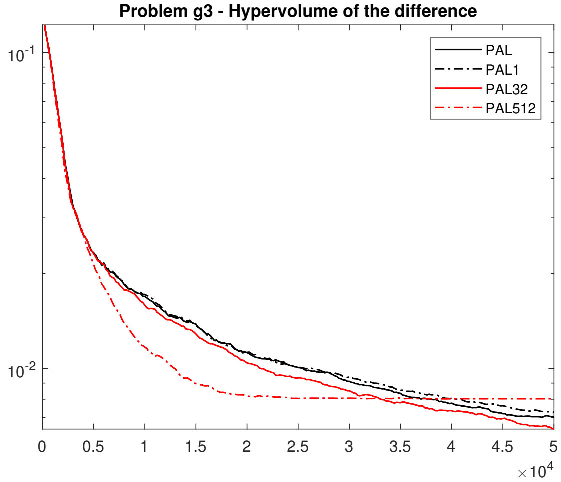


Figure 41: Average volume of the symmetric difference metric for problem $g_3$ for different $\varepsilon$ values.

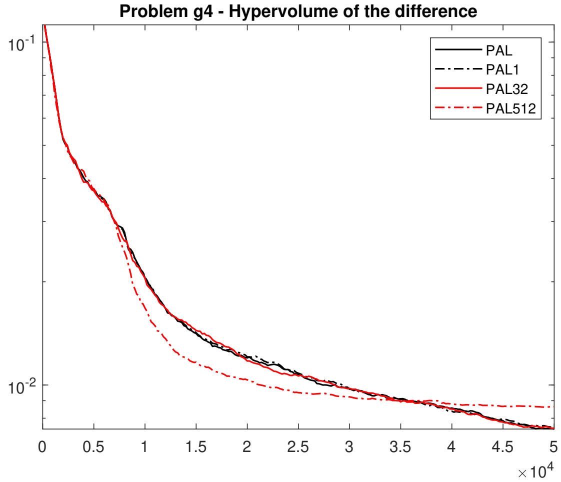


Figure 42: Average volume of the symmetric difference metric for problem $g_4$ for different $\varepsilon$ values.

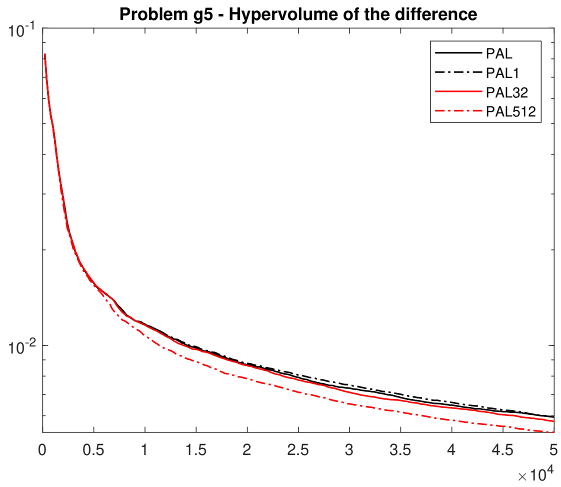


Figure 43: Average volume of the symmetric difference metric for problem $g_5$ for different $\varepsilon$ values.

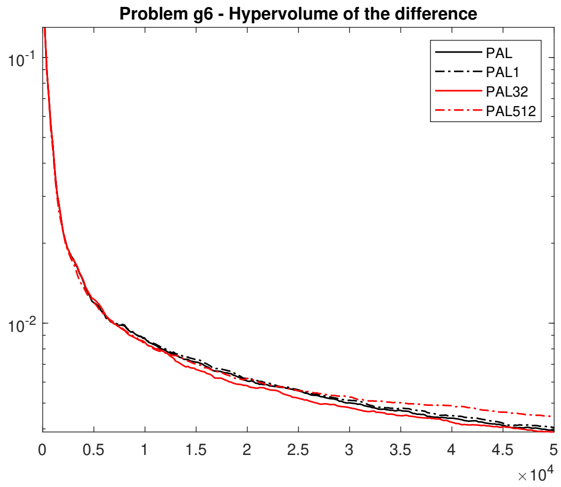


Figure 44: Average volume of the symmetric difference metric for problem $g_6$ for different $\varepsilon$ values.

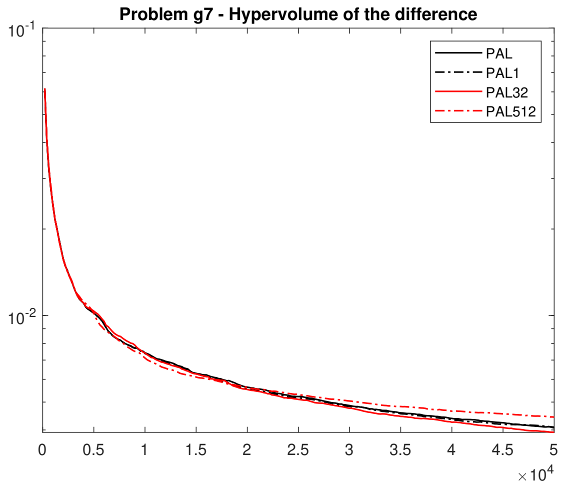


Figure 45: Average volume of the symmetric difference metric for problem $g_7$ for different $\varepsilon$ values.

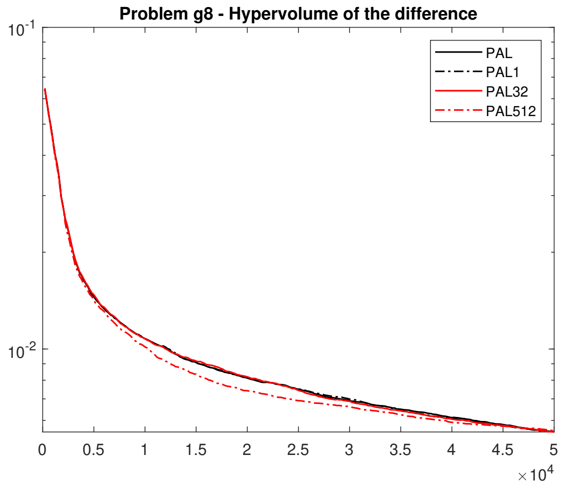


Figure 46: Average volume of the symmetric difference metric for problem $g_8$ for different $\varepsilon$ values.

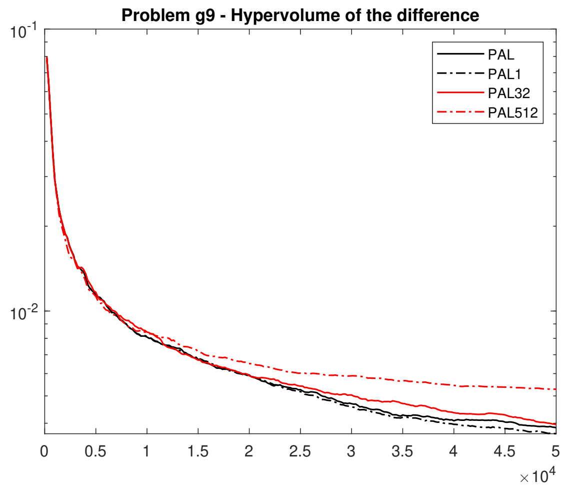


Figure 47: Average volume of the symmetric difference metric for problem $g_9$ for different $\varepsilon$ values.

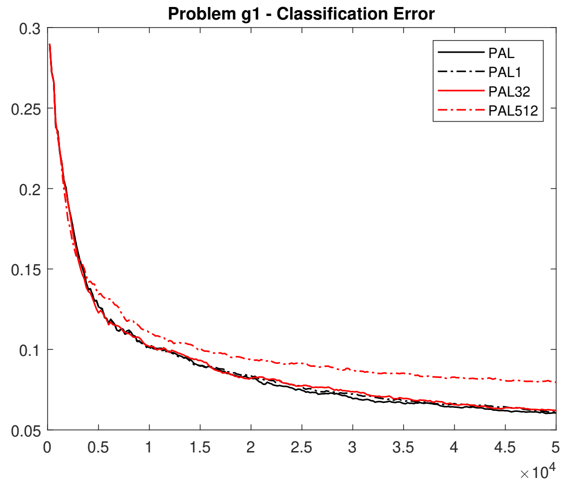


Figure 48: Average classification error metric for problem $g_1$ for different $\varepsilon$ values.

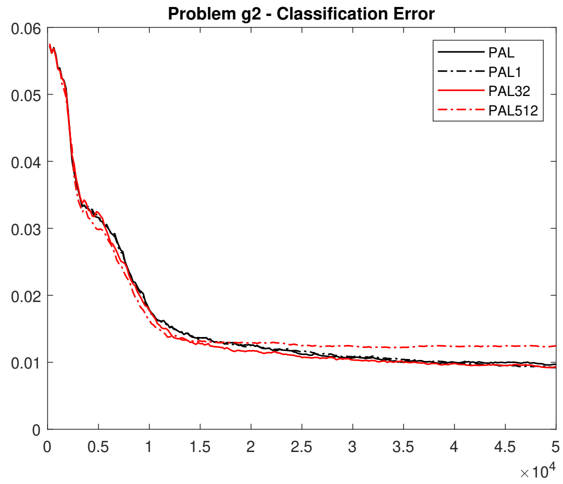


Figure 49: Average classification error metric for problem $g_2$ for different $\varepsilon$ values.

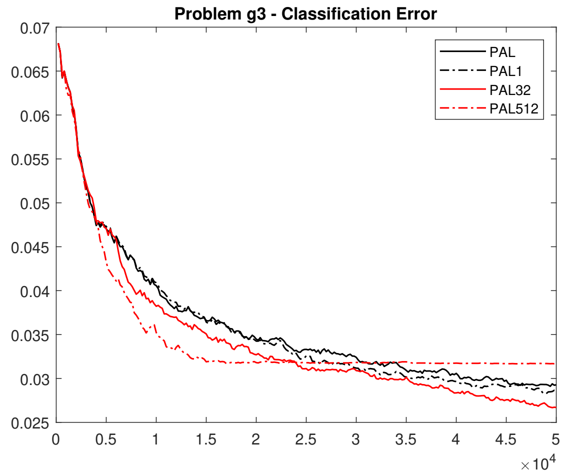


Figure 50: Average classification error metric for problem $g_3$ for different $\varepsilon$ values.

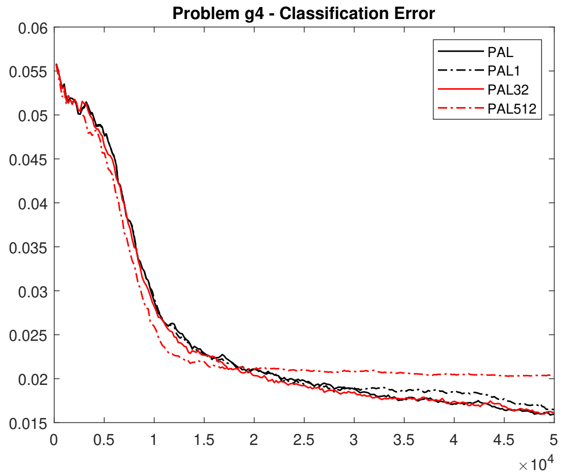


Figure 51: Average classification error metric for problem $g_4$ for different $\varepsilon$ values.

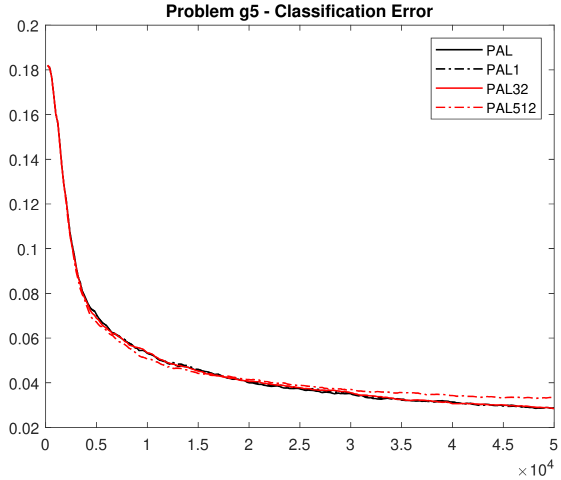


Figure 52: Average classification error metric for problem $g_5$ for different $\varepsilon$ values.

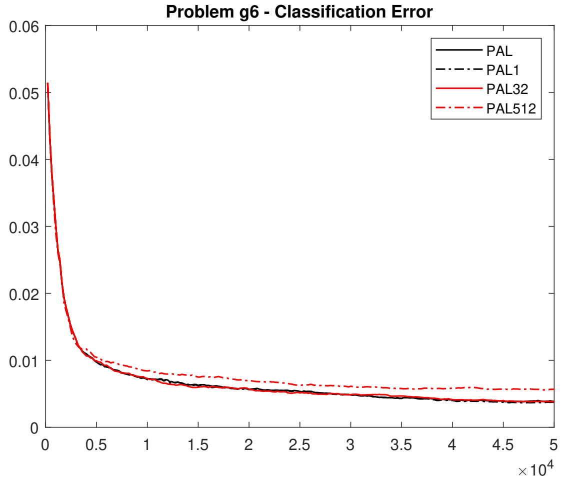


Figure 53: Average classification error metric for problem $g_6$ for different $\varepsilon$ values.

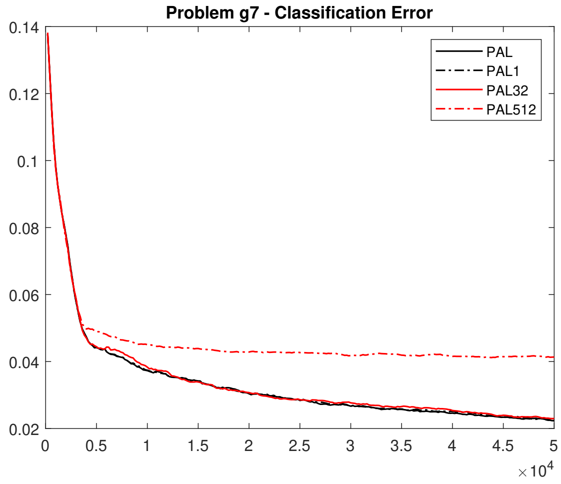


Figure 54: Average classification error metric for problem $g_7$ for different $\varepsilon$ values.

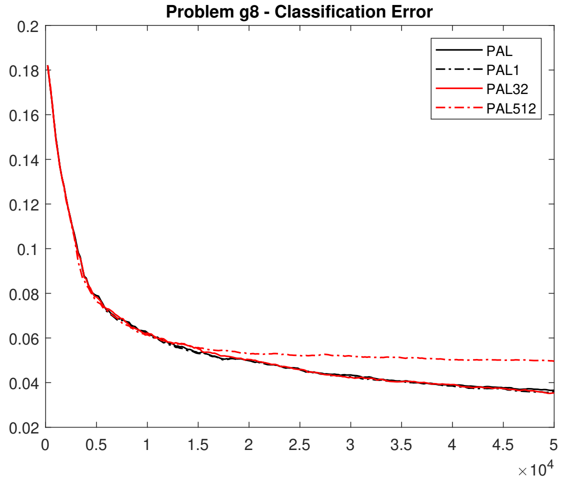


Figure 55: Average classification error metric for problem $g_8$ for different $\varepsilon$ values.

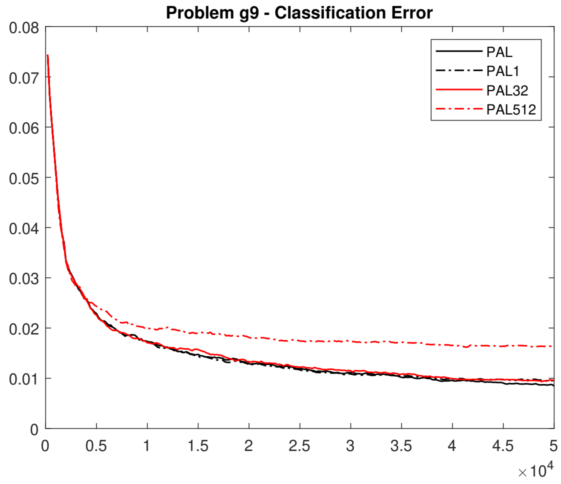


Figure 56: Average classification error metric for problem $g_9$ for different $\varepsilon$ values.

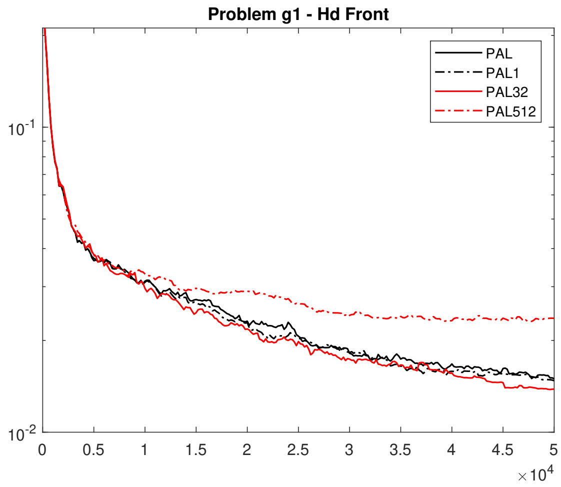


Figure 57: Average Hausdorff distance of the Pareto front prediction for problem $g_1$ for different $\varepsilon$ values.

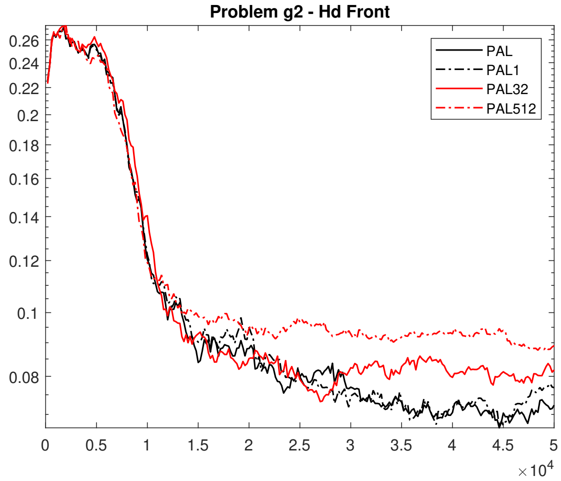


Figure 58: Average Hausdorff distance of the Pareto front prediction for problem $g_2$ for different $\varepsilon$ values.

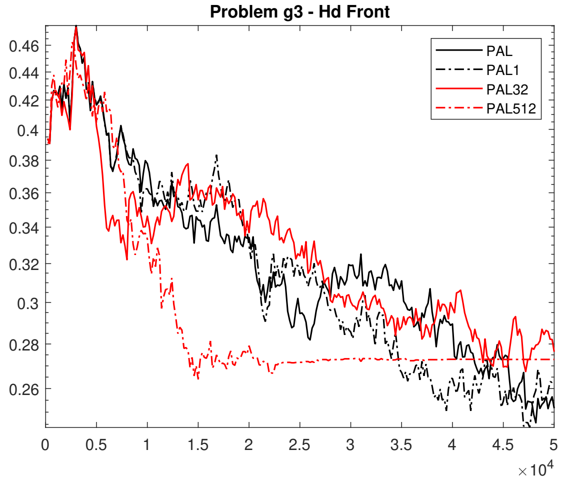


Figure 59: Average Hausdorff distance of the Pareto front prediction for problem $g_3$ for different $\varepsilon$ values.

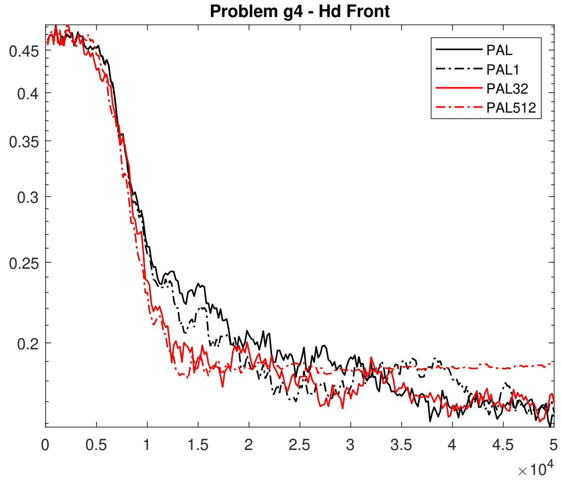


Figure 60: Average Hausdorff distance of the Pareto front prediction for problem $g_4$ for different $\varepsilon$ values.

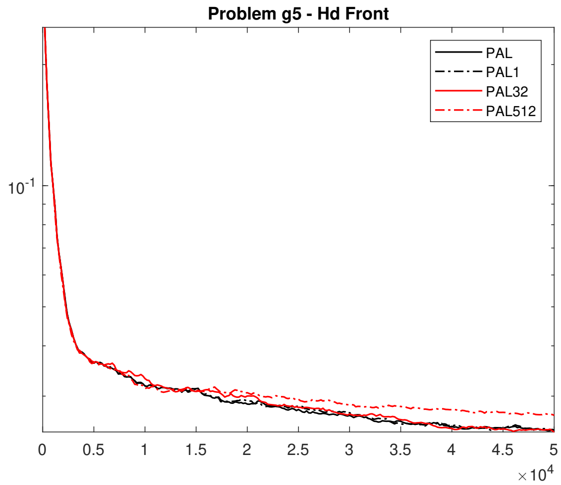


Figure 61: Average Hausdorff distance of the Pareto front prediction for problem $g_5$ for different $\varepsilon$ values.

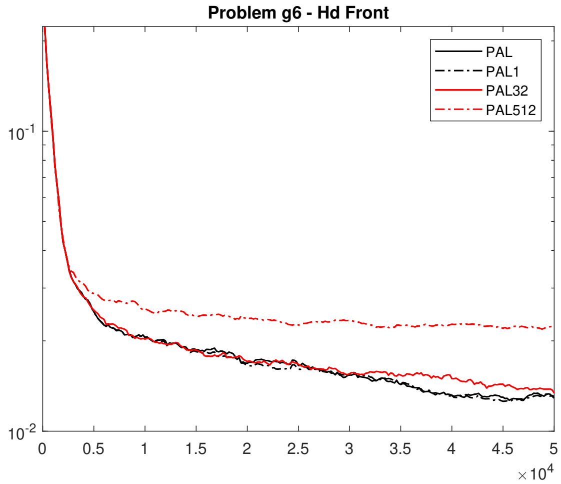


Figure 62: Average Hausdorff distance of the Pareto front prediction for problem $g_6$ for different $\varepsilon$ values.

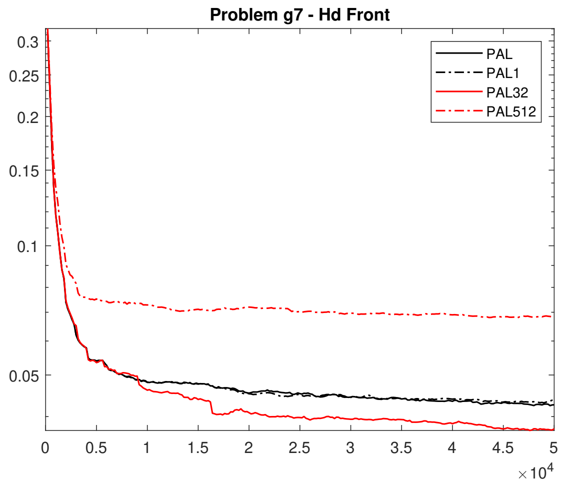


Figure 63: Average Hausdorff distance of the Pareto front prediction for problem $g_7$ for different $\varepsilon$ values.

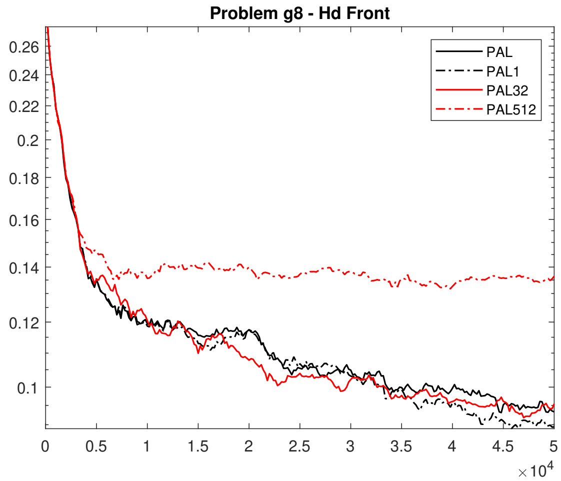


Figure 64: Average Hausdorff distance of the Pareto front prediction for problem $g_8$ for different $\varepsilon$ values.

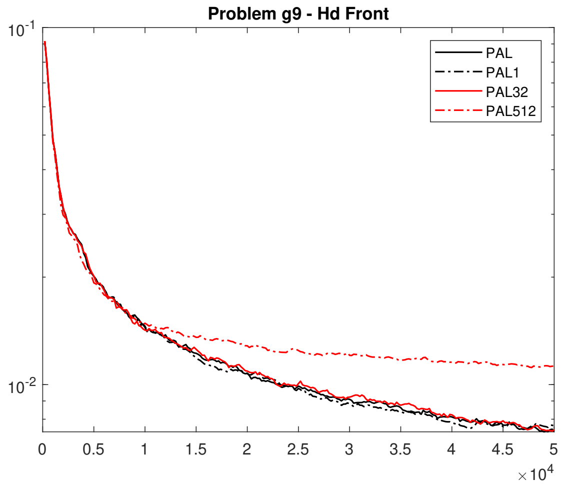


Figure 65: Average Hausdorff distance of the Pareto front prediction for problem $g_9$ for different $\varepsilon$ values.

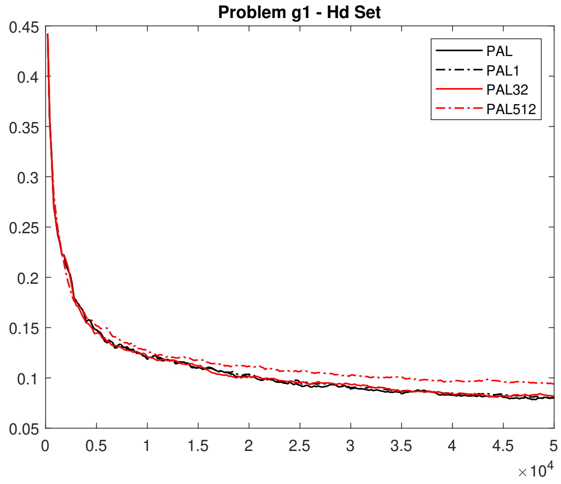


Figure 66: Average Hausdorff distance of the Pareto set prediction for problem $g_1$ for different $\varepsilon$ values.

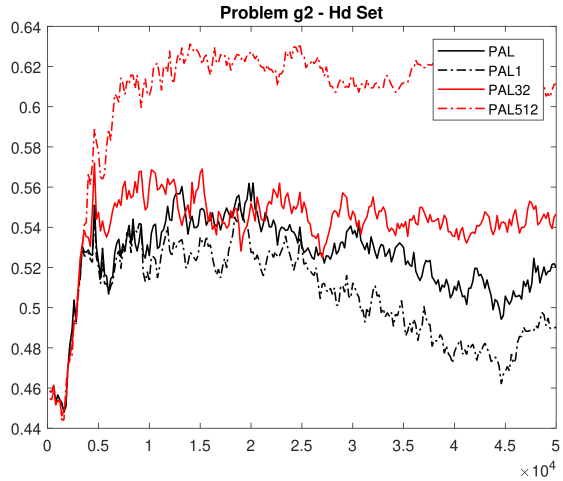


Figure 67: Average Hausdorff distance of the Pareto set prediction for problem $g_2$ for different $\varepsilon$ values.

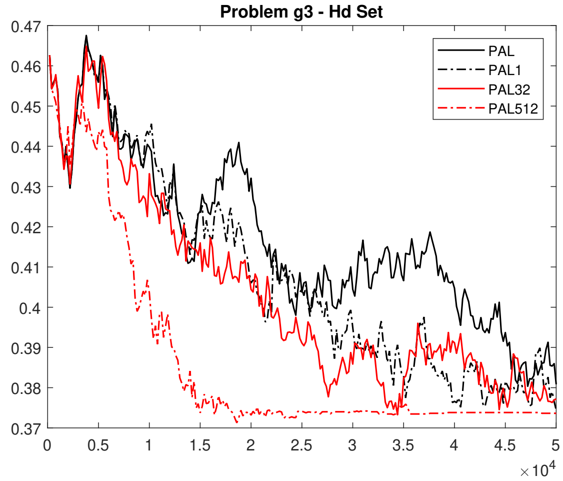


Figure 68: Average Hausdorff distance of the Pareto set prediction for problem $g_3$ for different $\varepsilon$ values.

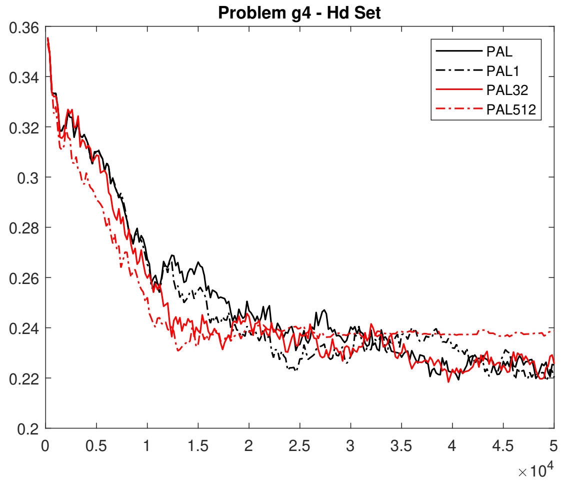


Figure 69: Average Hausdorff distance of the Pareto set prediction for problem $g_4$ for different $\varepsilon$ values.

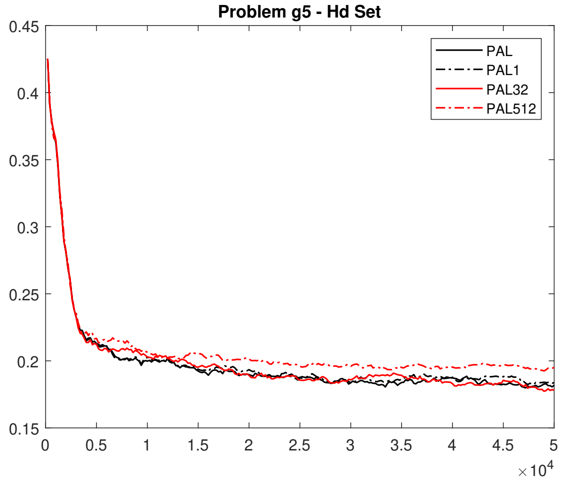


Figure 70: Average Hausdorff distance of the Pareto set prediction for problem $g_5$ for different $\varepsilon$ values.

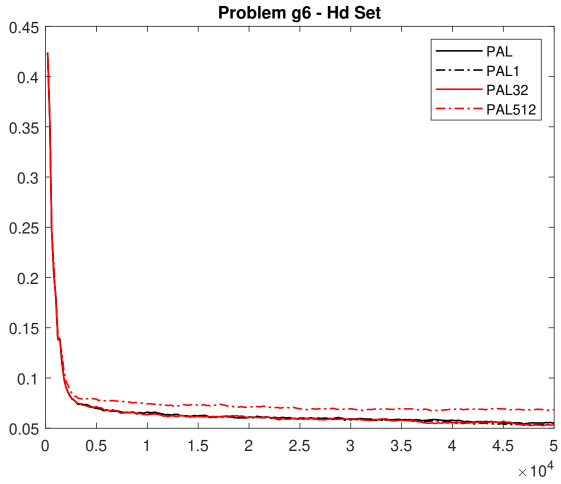


Figure 71: Average Hausdorff distance of the Pareto set prediction for problem $g_6$ for different $\varepsilon$ values.

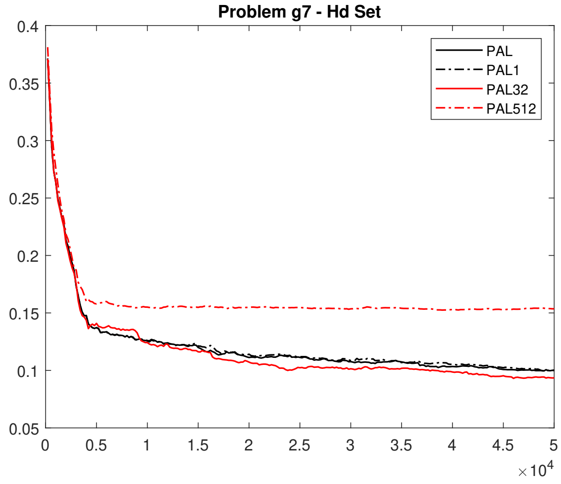


Figure 72: Average Hausdorff distance of the Pareto set prediction for problem $g_7$ for different $\varepsilon$ values.

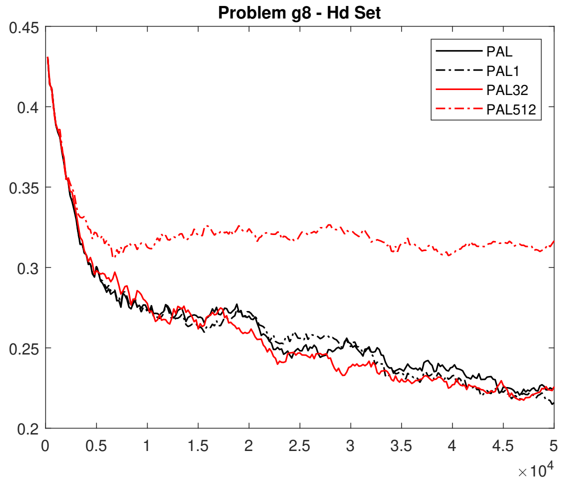


Figure 73: Average Hausdorff distance of the Pareto set prediction for problem $g_8$ for different $\varepsilon$ values.

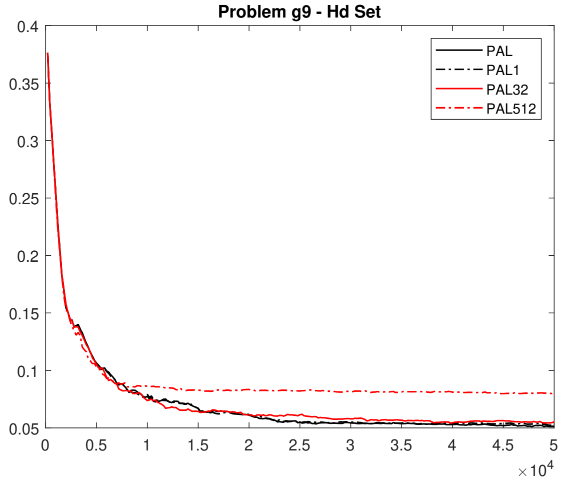


Figure 74: Average Hausdorff distance of the Pareto set prediction for problem $g_9$ for different $\varepsilon$ values.

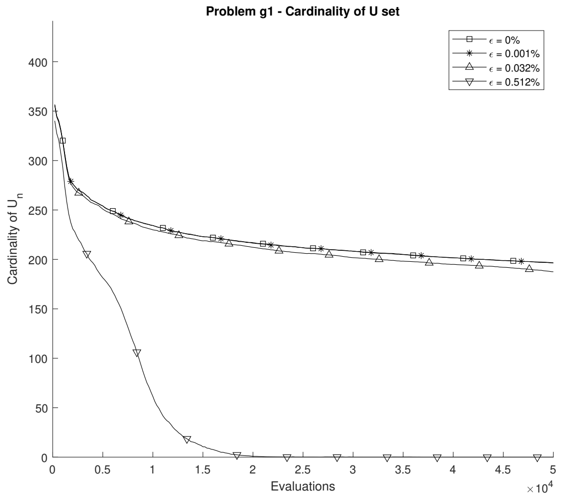


Figure 75: Average cardinality of the unclassified set for problem $g_1$ for different $\varepsilon$ values.

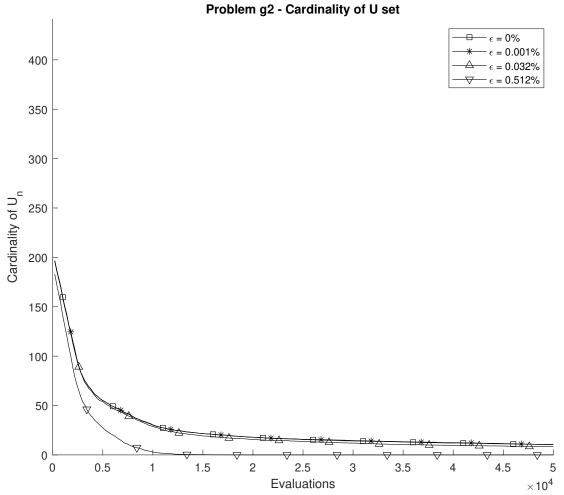


Figure 76: Average cardinality of the unclassified set for problem $g_2$ for different $\varepsilon$ values.

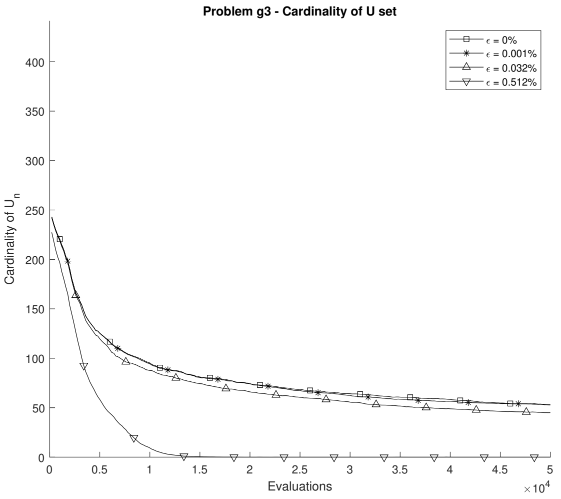


Figure 77: Average cardinality of the unclassified set for problem $g_3$ for different $\varepsilon$ values.

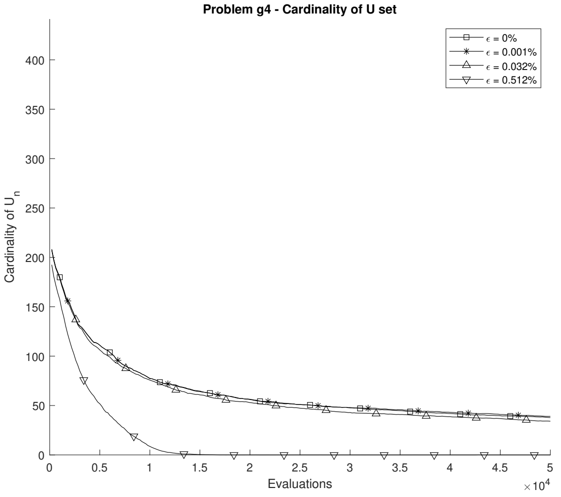


Figure 78: Average cardinality of the unclassified set for problem $g_4$ for different $\varepsilon$ values.

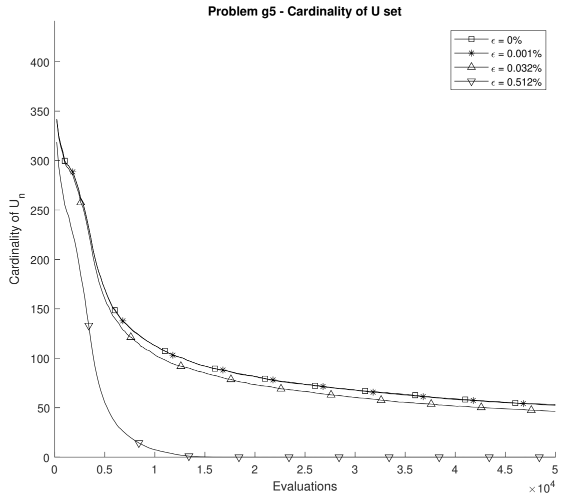


Figure 79: Average cardinality of the unclassified set for problem $g_5$ for different $\varepsilon$ values.

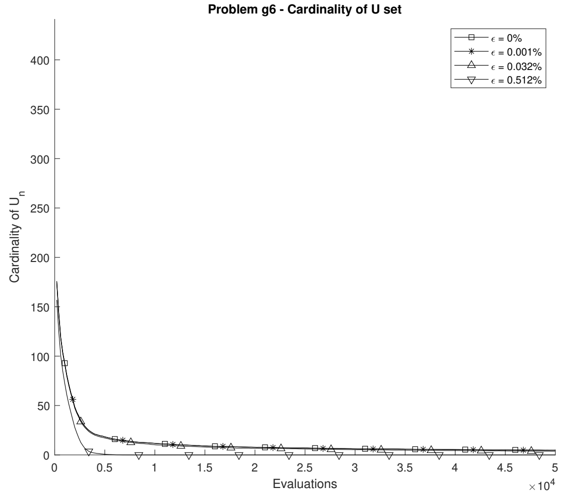


Figure 80: Average cardinality of the unclassified set for problem $g_6$ for different $\varepsilon$ values.

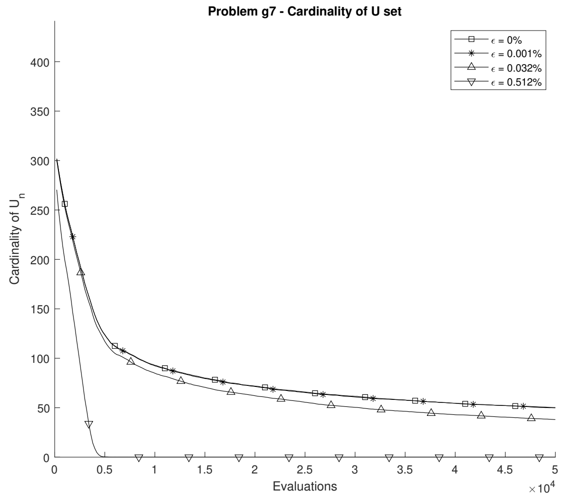


Figure 81: Average cardinality of the unclassified set for problem $g_7$ for different $\varepsilon$ values.

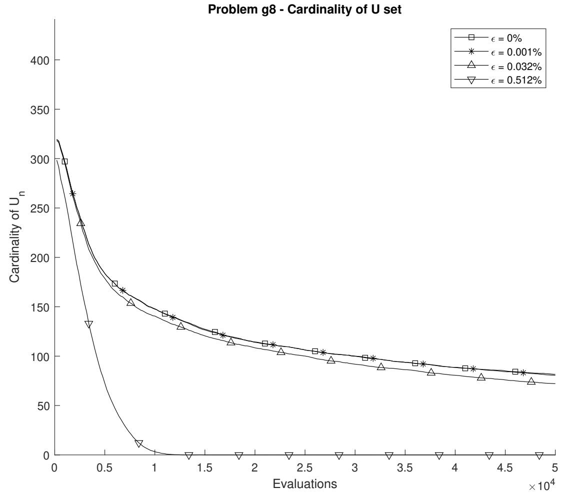


Figure 82: Average cardinality of the unclassified set for problem $g_8$ for different $\varepsilon$ values.

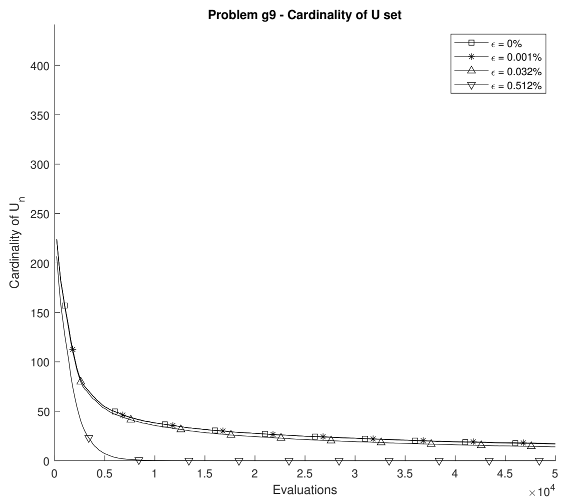


Figure 83: Average cardinality of the unclassified set for problem $g_9$ for different $\varepsilon$ values.

## 3. Using intersections in PALS

Figure 84 presents the ratio of average metric values for volume of the symmetric difference (left) and classification error (right), when compared to the random approach, for the situations where half the budget us used (circles) and total budget (diamonds). What is observed is that intersections do not improve the algorithm efficiency at neither stages of the process.

If instead of considering the average metrics, we look at the metric value at each of the experiments, for each problem, for the volume of the symmetric difference (Figure 85) and for the clssification error (Figure 86) we obtain similar conclusions. The fact that the scatter plots present symmetric clouds around the diagonal dashed line indicate that there seems to be no interest to adopt one of the methods when compared to the other.

Considering these numerical experiment results, it seems to be no interest in the use of intersection in the PALS algorithm, given that it bring no advantage and can generate problems in the algorithm execution.

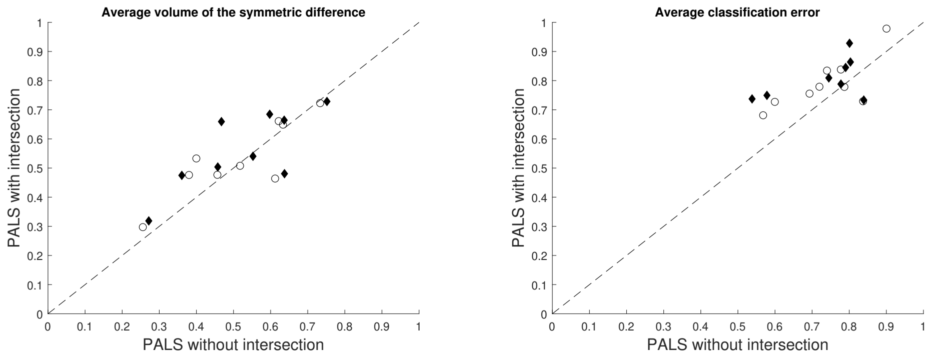


Figure 84: Ratio comparison between PALS algorithm performance (with and without intersection) and a random approach. Average hypervolume difference (left) and classification error (right) considering 500 random initialization, obtained after a budget of 25000 evaluations (circles) and 50000 evaluations (diamonds).

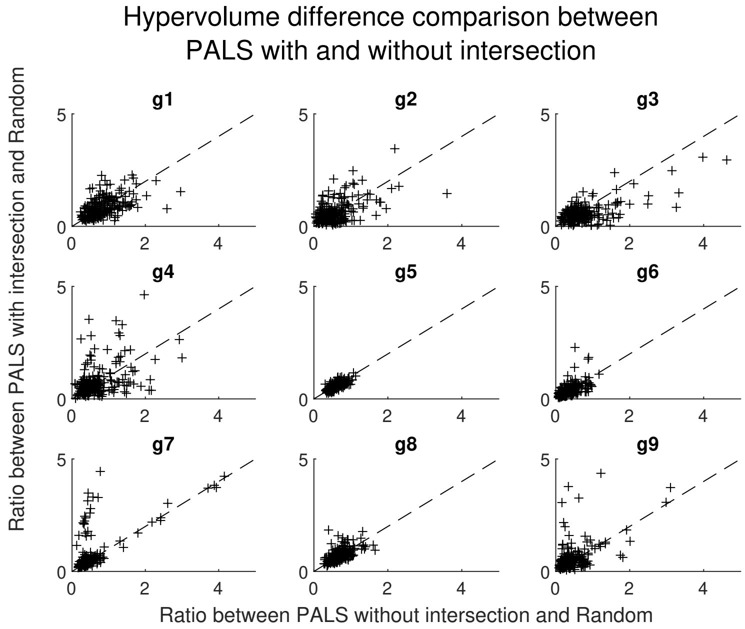


Figure 85: Ratio comparison between PALS algorithm performance (with and without intersection) and a random approach for all problems. Hypervolume difference for each of the 500 random initialization, obtained after a budget of 50000 evaluations.

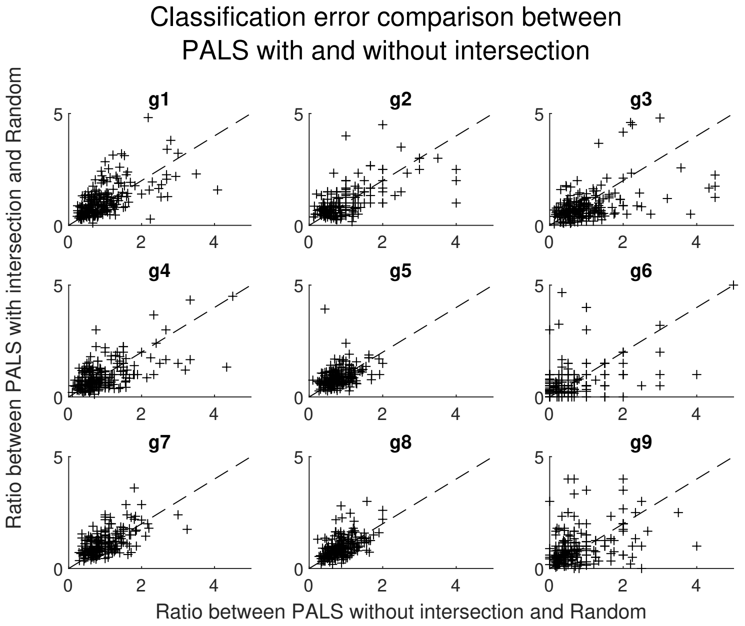


Figure 86: Ratio comparison between PALS algorithm performance (with and without intersection) and a random approach for all problems. Classification error for each of the 500 random initialization, obtained after a budget of 50000 evaluations.

## 4. Influence of the batch size

A comparison between the use of batches of 200, 500, 1000, and 2000 evaluations is performed. For the classification error metric results are presented on Figures 87 to 87.

For the average hypervolume metric results are presented on Figures 96 to 96.

We observe clearly that, although the batch size choice has no impact at the final iteration average metric value, the smaller batch size presents better results at early phases.

We can assume that a smaller batch size allows an initial stage space exploration that increases the quality of the prediction models. However, in all observed cases, at a final stage no significant differences were observed.

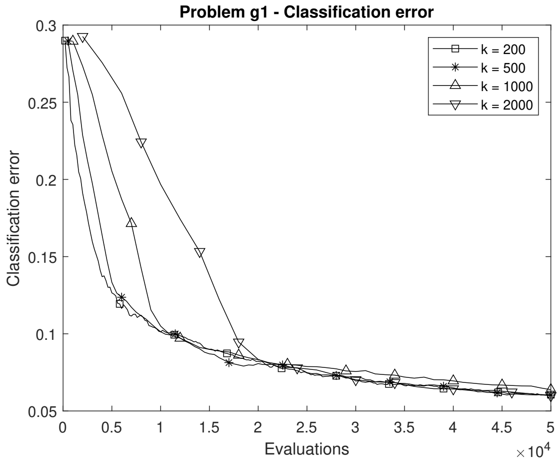


Figure 87: Average classification error comparison for problem $g_1$ when considering $k$ of 200, 500, 1000 and 2000.

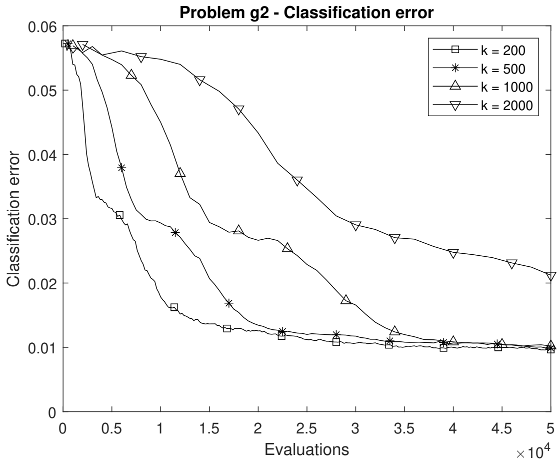


Figure 88: Average classification error comparison for problem $g_2$ when considering $k$ of 200, 500, 1000 and 2000.

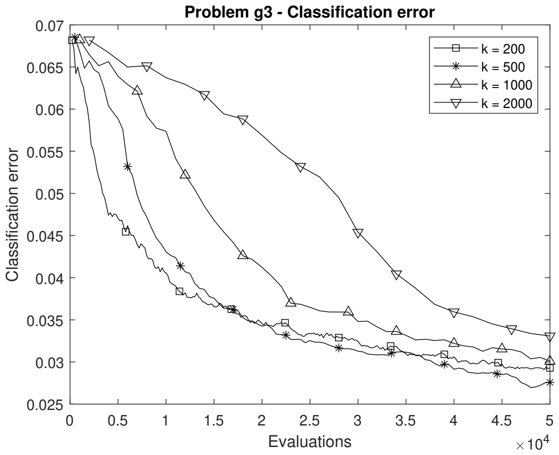


Figure 89: Average classification error comparison for problem $g_3$ when considering $k$ of 200, 500, 1000 and 2000.

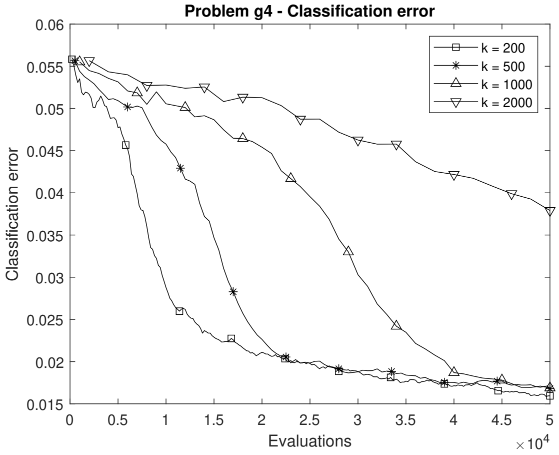


Figure 90: Average classification error comparison for problem $g_4$ when considering $k$ of 200, 500, 1000 and 2000.

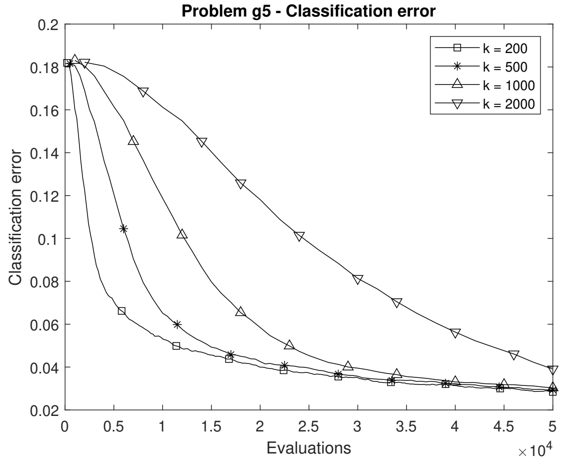


Figure 91: Average classification error comparison for problem $g_5$ when considering $k$ of 200, 500, 1000 and 2000.

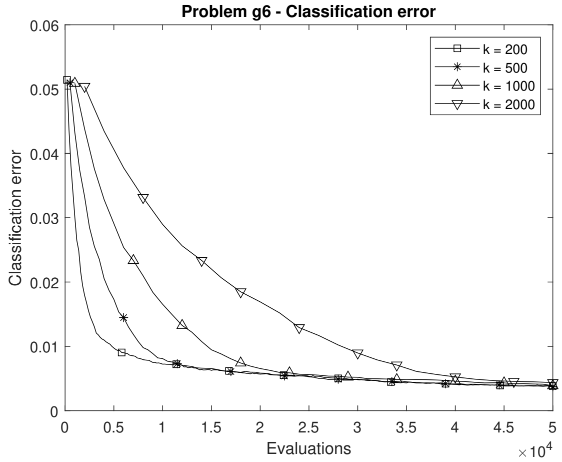


Figure 92: Average classification error comparison for problem $g_6$ when considering $k$ of 200, 500, 1000 and 2000.

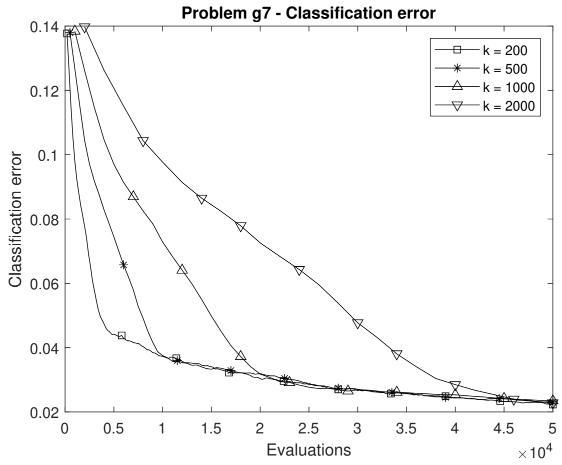


Figure 93: Average classification error comparison for problem $g_7$ when considering $k$ of 200, 500, 1000 and 2000.

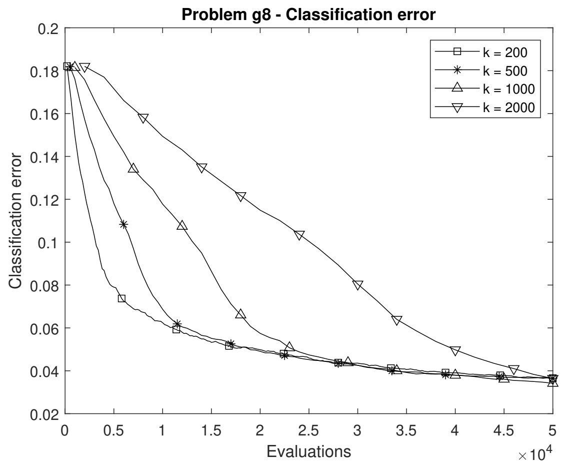


Figure 94: Average classification error comparison for problem $g_8$ when considering $k$ of 200, 500, 1000 and 2000.

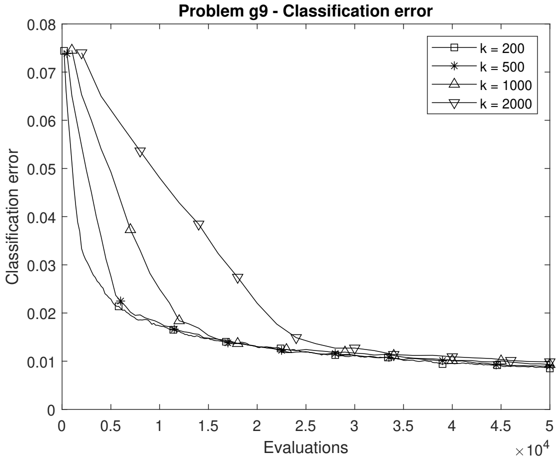


Figure 95: Average classification error comparison for problem $g_9$ when considering $k$ of 200, 500, 1000 and 2000.

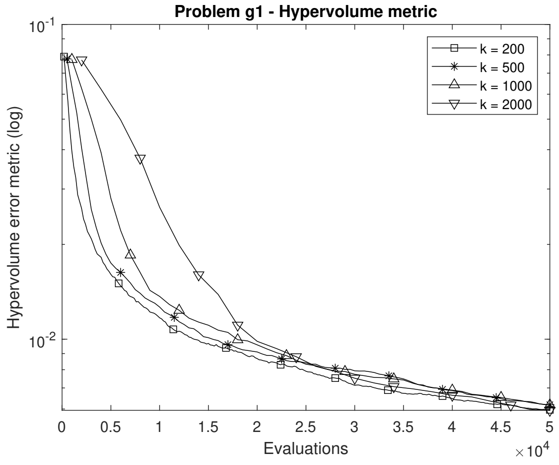


Figure 96: Average hypervolume error comparison for problem $g_1$ when considering $k$ of 200, 500, 1000 and 2000.

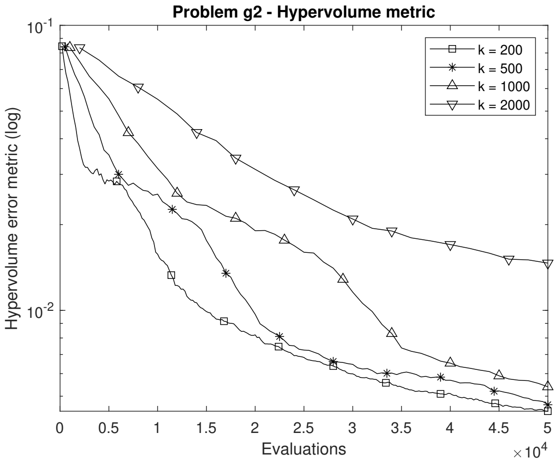


Figure 97: Average hypervolume error comparison for problem $g_2$ when considering $k$ of 200, 500, 1000 and 2000.

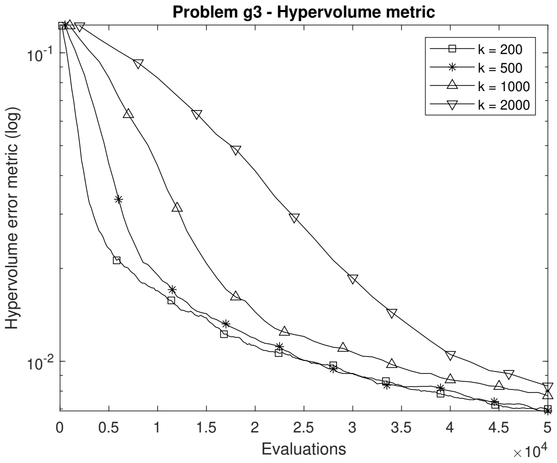


Figure 98: Average hypervolume error comparison for problem $g_3$ when considering $k$ of 200, 500, 1000 and 2000.

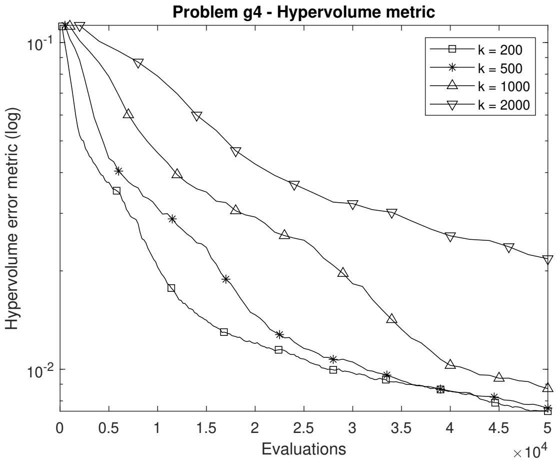


Figure 99: Average hypervolume error comparison for problem $g_4$ when considering $k$ of 200, 500, 1000 and 2000.

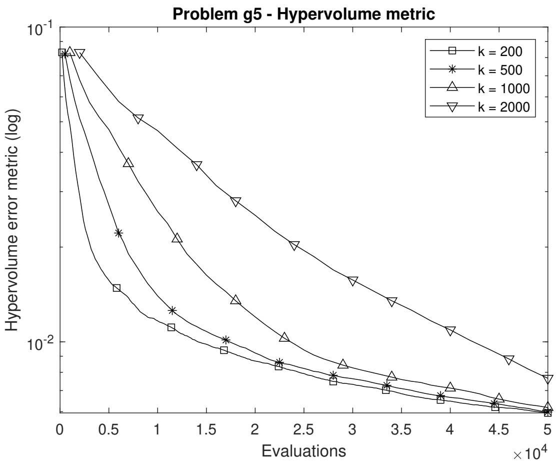


Figure 100: Average hypervolume error comparison for problem $g_5$ when considering $k$ of 200, 500, 1000 and 2000.

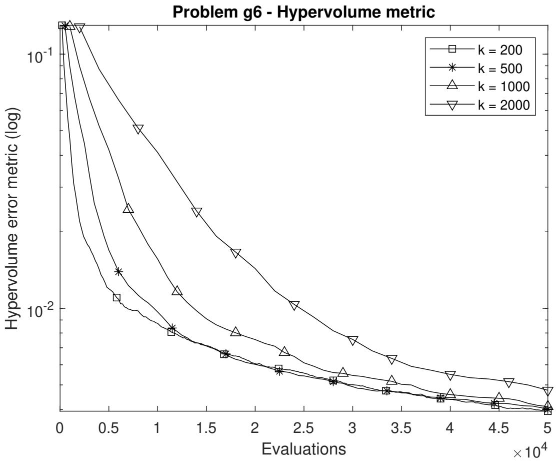


Figure 101: Average hypervolume error comparison for problem $g_6$ when considering $k$ of 200, 500, 1000 and 2000.

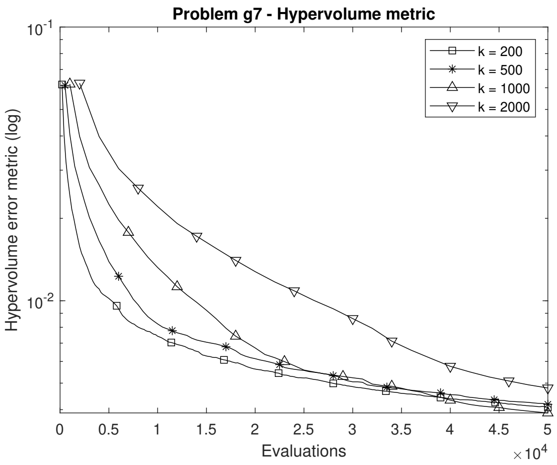


Figure 102: Average hypervolume error comparison for problem $g_7$ when considering $k$ of 200, 500, 1000 and 2000.

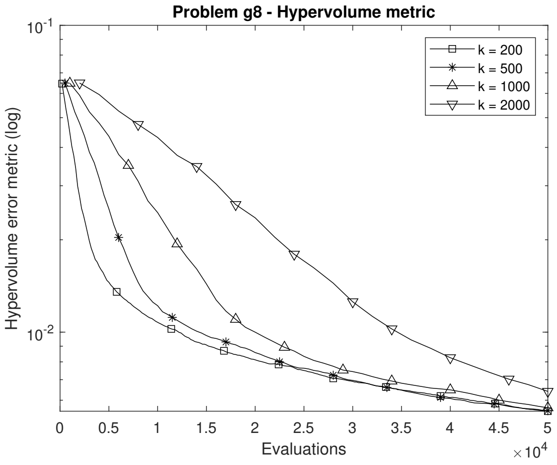


Figure 103: Average hypervolume error comparison for problem $g_8$ when considering $k$ of 200, 500, 1000 and 2000.

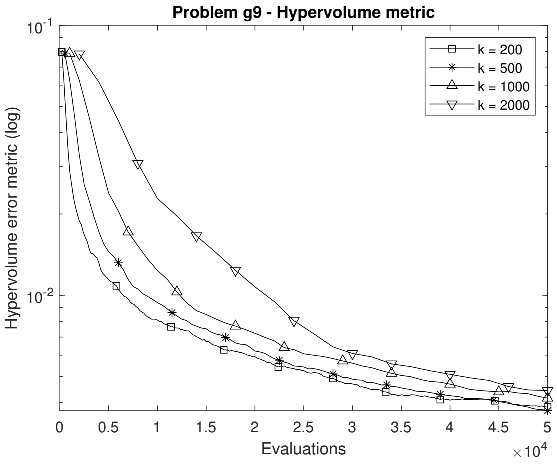


Figure 104: Average hypervolume error comparison for problem $g_9$ when considering $k$ of 200, 500, 1000 and 2000.

## 5. Comparison of two random-based proposed alternatives

As proposed in the original article, two alternative random approaches are considered. We considered an approach based on selecting points randomly proportional to the probability of misclassification and as an alternative, proporcional to the probability of non-domination. Figure 105 presents a scatter plot comparing the ratios between those approaches and a random approach.

Points placed close to the diagonal dashed line imply that the performance was similar for both approaches. While there is no significant difference for the classification error metric (right), we can see that for some of the test problems the volume of the symmetric difference metric (left) shows a better performance of the probability of non-domination approach. For the numerical experiments we name this approach “Concentrated” Random Sampling.

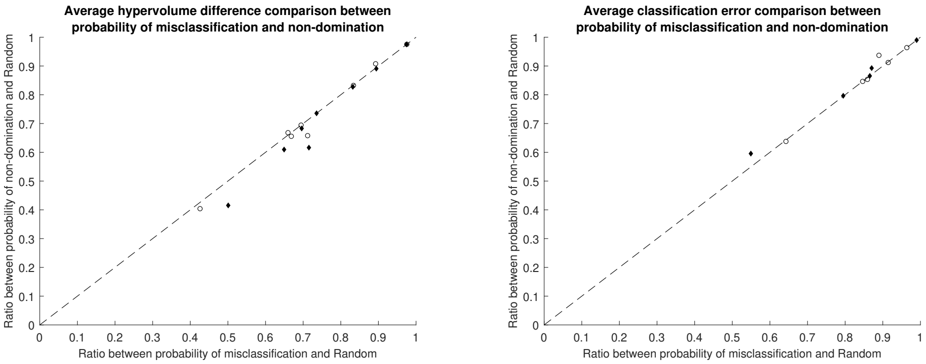


Figure 105: Ratio comparison between alternative random approaches performance (based on probability of misclassification and probability of non-domination) and a random approach. Average hypervolume difference (left) and classification error (right) considering 500 random initialization, obtained after a budget of 25000 evaluations (circles) and 50000 evaluations (diamonds).

## 6. Comparison with other approaches

Figures 106 to 114 present the average performance metrics volume of the symmetric difference for test problems $g_1$ to $g_9$. Comparison is presented between random approach, “Concentrated” Random Sampling, $EI_m$ and PALS.

A similar comparison is presented for classification error metrics on Figures 115 to 123

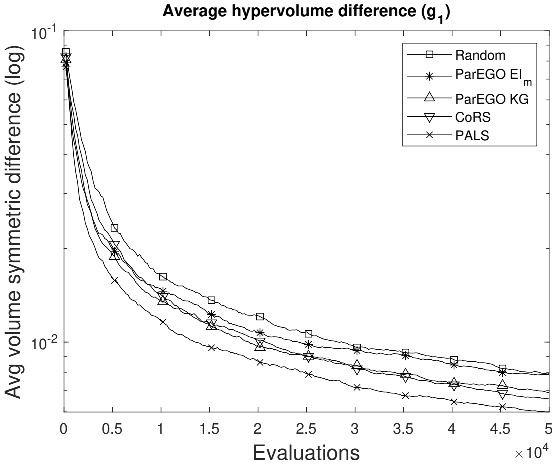


Figure 106: Average hypervolume difference for test problem $g_1$. Comparison between random approach, “Concentrated” Random Sampling, $EI_m$ and PALS.

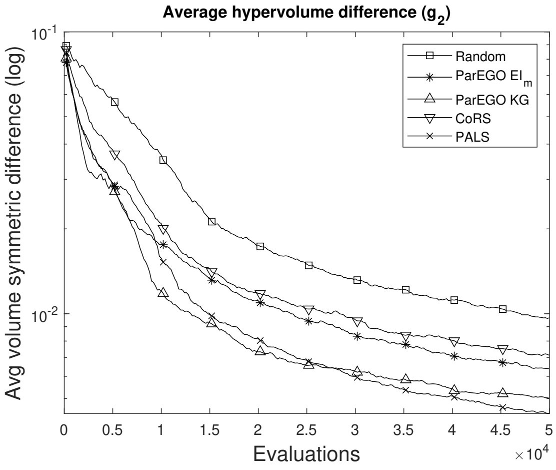


Figure 107: Average hypervolume difference for test problem $g_2$. Comparison between random approach, “Concentrated” Random Sampling, $EI_m$ and PALS.

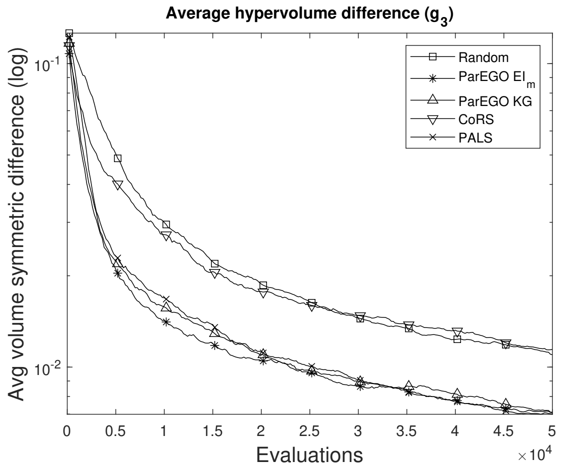


Figure 108: Average hypervolume difference for test problem $g_3$. Comparison between random approach, "Concentrated" Random Sampling, $EI_m$ and PALS.

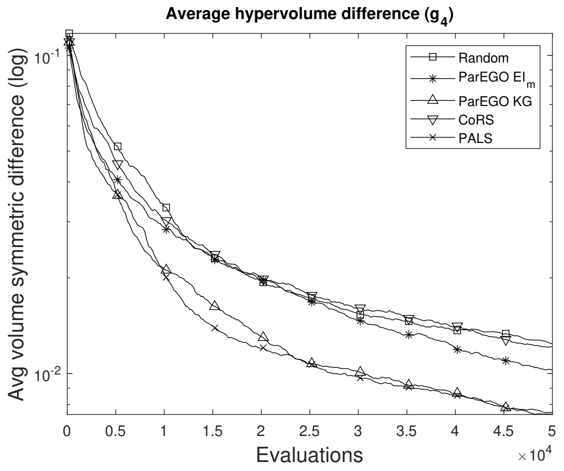


Figure 109: Average hypervolume difference for test problem $g_4$. Comparison between random approach, "Concentrated" Random Sampling, $EI_m$ and PALS.

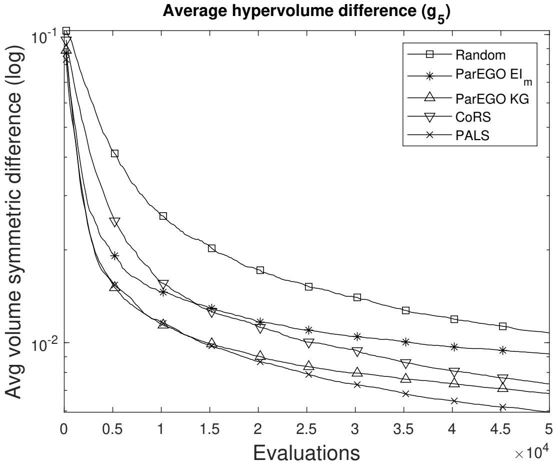


Figure 110: Average hypervolume difference for test problem $g_5$. Comparison between random approach, "Concentrated" Random Sampling, $EI_m$ and PALS.

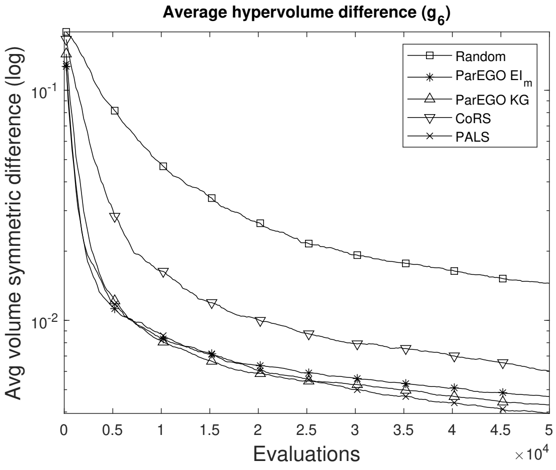


Figure 111: Average hypervolume difference for test problem $g_6$. Comparison between random approach, "Concentrated" Random Sampling, $EI_m$ and PALS.

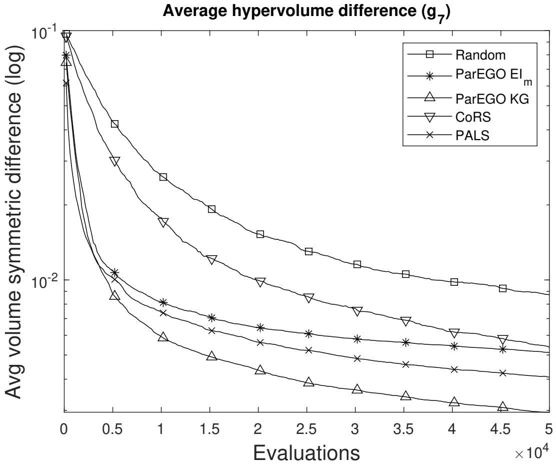


Figure 112: Average hypervolume difference for test problem $g_7$. Comparison between random approach, "Concentrated" Random Sampling, $EI_m$ and PALS.

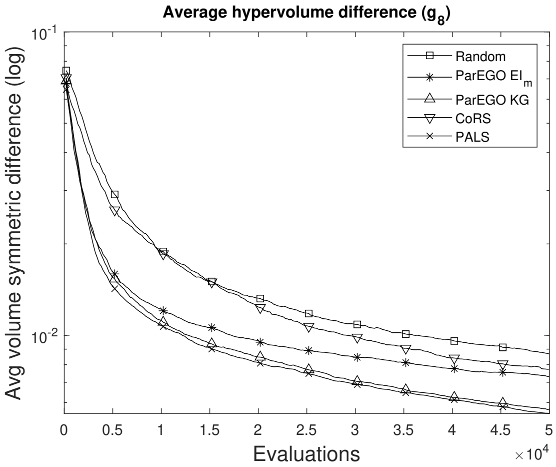


Figure 113: Average hypervolume difference for test problem $g_8$. Comparison between random approach, "Concentrated" Random Sampling, $EI_m$ and PALS.

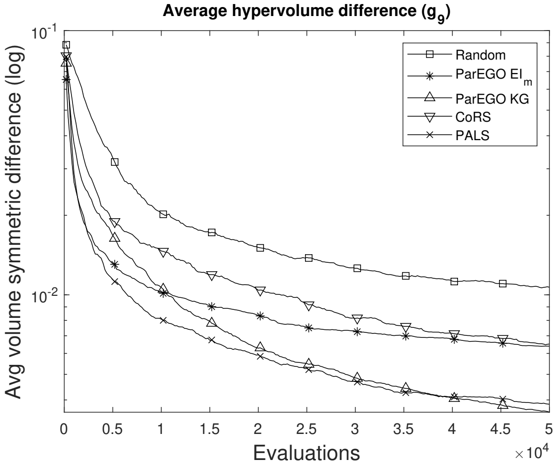


Figure 114: Average hypervolume difference for test problem $g_9$. Comparison between random approach, "Concentrated" Random Sampling, $EI_m$ and PALS.

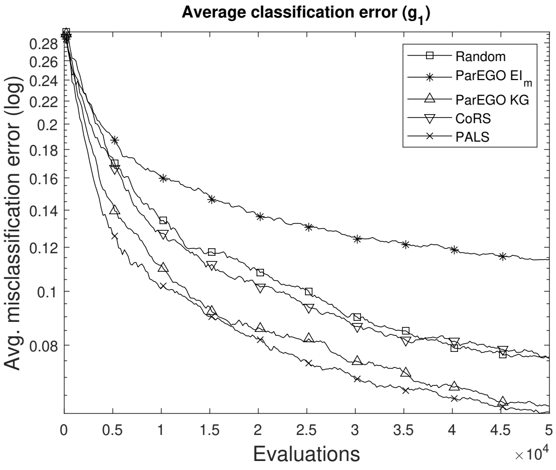


Figure 115: Average classification error for test problem $g_1$. Comparison between random approach, "Concentrated" Random Sampling, $EI_m$ and PALS.

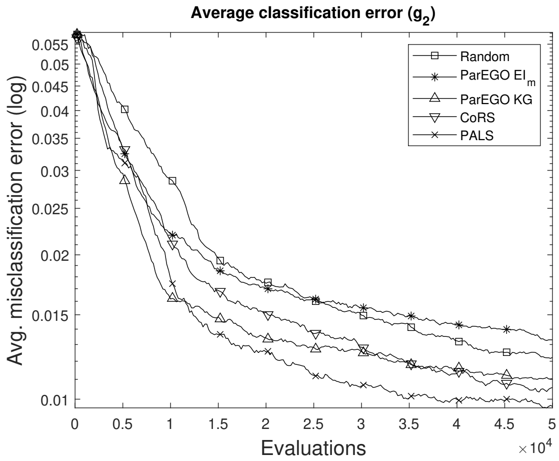


Figure 116: Average classification error for test problem $g_2$. Comparison between random approach, "Concentrated" Random Sampling, $EI_m$ and PALS.

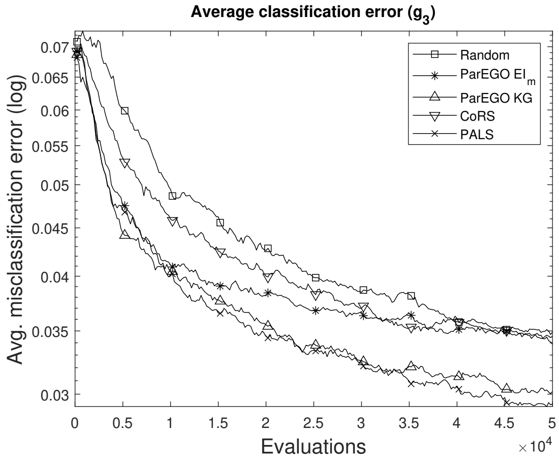


Figure 117: Average classification error for test problem $g_3$. Comparison between random approach, "Concentrated" Random Sampling, $EI_m$ and PALS.

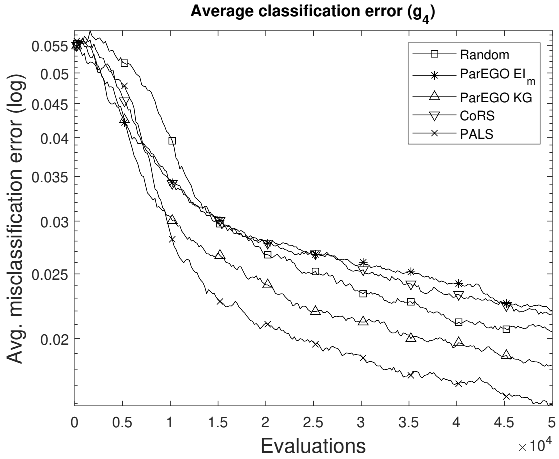


Figure 118: Average classification error for test problem $g_4$. Comparison between random approach, "Concentrated" Random Sampling, $EI_m$ and PALS.

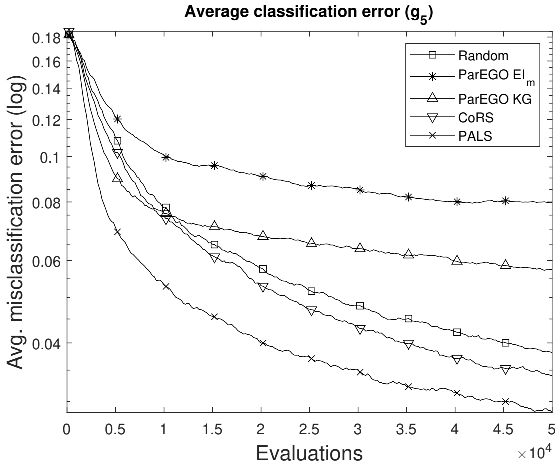


Figure 119: Average classification error for test problem $g_5$. Comparison between random approach, "Concentrated" Random Sampling, $EI_m$ and PALS.

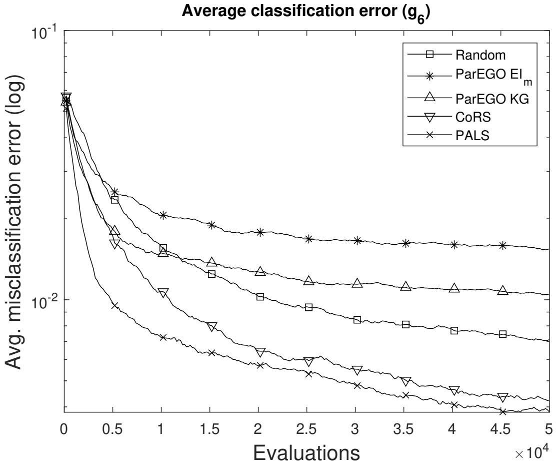


Figure 120: Average classification error for test problem $g_6$. Comparison between random approach, "Concentrated" Random Sampling, $EI_m$ and PALS.

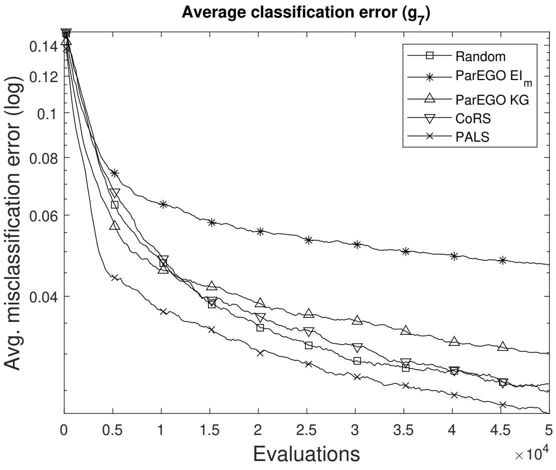


Figure 121: Average classification error for test problem $g_7$. Comparison between random approach, "Concentrated" Random Sampling, $EI_m$ and PALS.

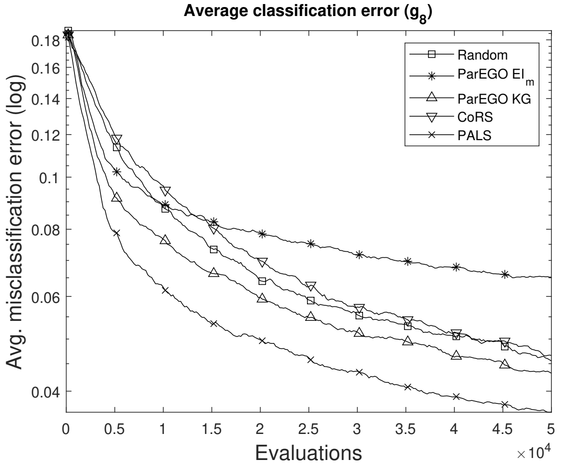


Figure 122: Average classification error for test problem $g_8$. Comparison between random approach, "Concentrated" Random Sampling, $EI_m$ and PALS.

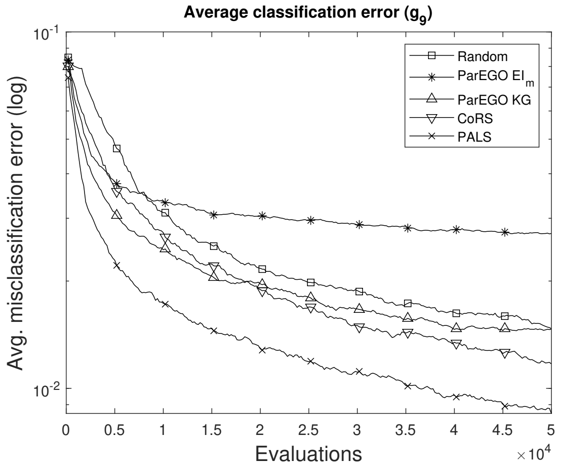


Figure 123: Average classification error for test problem $g_9$. Comparison between random approach, "Concentrated" Random Sampling, $EI_m$ and PALS.
